# Supplementary material for: The complexity of dynamics in small neural circuits
Source: arXiv:1506.08995 ancillary file (2015-07-22)
Supplement: Supplementary file 1 [file Supplementary_Materials.pdf]

# Supplementary Materials to: The complexity of dynamics in small neural circuits

Diego Fasoli[1,*], Anna Cattani[1], Stefano Panzeri[1]

**1 Neural Computation Laboratory, Center for Neuroscience and Cognitive Systems @Unitn, Istituto Italiano di Tecnologia, 38068 Rovereto (Tn), Italy**

$*$ **E-mail: diego.fasoli@iit.it**

## S1 Introduction

In this article we present the Supplementary Materials to [1]. In order to make the mathematical part of this text as linear as possible, in some sections we repeat the derivations we already introduced in [1], and then we analyze them in more detail. On the other side, the remaining sections are completely new and self-contained.

This work is organized as follows. First, in Sec. (S2) we partially calculate the codimension one bifurcation diagram of the network by evaluating the equilibrium points on the primary branch. This calculation is based on an asymptotic perturbative expansion of the neural equations, so it provides a good description of the membrane potentials in the stationary regime only for sufficiently large values of $I_E$ (see Eqs. (5) and (10) in [1]), where the branching point bifurcations do not occur. Then, as in [1], we divide the second part of the Supplementary Materials in two main sections, devoted to the study of weak (Sec. (S3)) and strong inhibition (Sec. (S4)). In both the cases we present detailed analytical calculations of the eigenvalues of the Jacobian matrix and of the codimension two bifurcation diagram for most of the local bifurcations of the network. Since the perturbative expansion introduced in Sec. (S2) cannot be extended to derive the secondary branches, a complete picture of the codimension one bifurcation diagram cannot be derived analytically. For this reason we conclude the Supplementary Materials by showing, in Sec. (S5), some panels of the codimension one bifurcations obtained by means of numerical tools, in order to further clarify the dynamics the model exhibits. As usual, all the results are obtained for the values of the parameters shown in Tab. (1).

## S2 Equilibrium points (codimension one bifurcation diagram)

In this section we study analytically the equilibrium points of the neural network. From the top-right panel of Fig. (2), we can see that some of the solutions of the system (5) (or, equivalently, of the system (10) with $\mu_{I,0} = \ldots \mu_{I,N_I-1} \stackrel{\mathrm{def}}{=} \mu_I$, namely on the primary branch) occur when at least one of the two nullclines is approximately constant in the phase space. For example, if we call $\mu_E = f(\mu_I)$ the implicit function obtained by solving the equation $\mathscr{F}(\mu_E, \mu_I) = 0$, from the top-right panel of Fig. (2) it is clear that two stationary solutions are obtained when $f(\cdot)$ is approximately constant in $\mu_I$ (see the vertical portions of the violet curves). In turn, this means that $\mathscr{A}_I(\mu_I)$ is approximately constant, namely the sigmoid function saturates to 0 or $\nu_I^{\max}$. Now we consider the case of saturation to $\nu_I^{\max}$ (the case of saturation to zero will be considered briefly later in this section), so in order to find the solutions of the systems (5) or (10) on the vertical portion of $f(\cdot)$, we need an asymptotic expansion of $\mathscr{A}_I(\mu_I)$ when $\mu_I \to +\infty$. If we use, as in [1], the algebraic activation function:

$$\mathscr{A}_{\alpha}\left(V\right)=\frac{\nu_{\alpha}^{\max}}{2}\left[1+\frac{\frac{\Lambda_{\alpha}}{2}\left(V-V_{\alpha}^{T}\right)}{\sqrt{1+\frac{\Lambda_{\alpha}^{2}}{4}\left(V-V_{\alpha}^{T}\right)^{2}}}\right] \tag{S1}$$

then we need an asymptotic expansion of:

$$\frac{x}{\sqrt{1+x^{2}}}=\frac{1}{\sqrt{1+y^{2}}}$$

(with $x=\frac{\Lambda_{I}}{2}\left(\mu_{I}-V_{I}^{T}\right)$ and $y=\frac{1}{x}$), about the point $y=0^{+}$ (i.e. $x=+\infty$). Since:

$$\frac{1}{\sqrt{1+y^{2}}}=\sum_{n=0}^{\infty}\left(-1\right)^{n}\frac{\left(2n-1\right)!!}{\left(2n\right)!!}y^{2n}=1-\frac{1}{2}y^{2}+\frac{1\cdot3}{2\cdot4}y^{4}-\frac{1\cdot3\cdot5}{2\cdot4\cdot6}y^{6}+\ldots$$

then, if we consider the expansion up to the first order, we can approximate $\mathscr{A}_{I}\left(\mu_{I}\right)$ as follows:

$$\mathscr{A}_{I}\left(\mu_{I}\right)\approx\frac{\nu_{I}^{\max}}{2}\left(1+1-\frac{1}{2x^{2}}\right)=\nu_{I}^{\max}\left(1-\frac{1}{4x^{2}}\right)$$

In a similar way, we suppose that also $\mu_{E}$ could be expanded in an asymptotic series, namely:

$$\mu_{E}=\sum_{n=0}^{\infty}\frac{\mu_{E}^{(n)}}{x^{2n}}$$

In particular, here we consider only the first two terms of this expansion, since they are sufficient to describe locally the equilibrium points of the primary branch with a good approximation. Therefore $\mathscr{A}_{E}\left(\mu_{E}\right)$ can be written as follows:

$$\mathscr{A}_{E}\left(\mu_{E}\right)\approx\mathscr{A}_{E}\left(\mu_{E}^{(0)}+\frac{\mu_{E}^{(1)}}{x^{2}}\right)\approx\mathscr{A}_{E}\left(\mu_{E}^{(0)}\right)+\mathscr{A}_{E}'\left(\mu_{E}^{(0)}\right)\frac{\mu_{E}^{(1)}}{x^{2}}$$

where at the second step we have used a Taylor expansion. With these assumptions, the system (5) (or equivalently (10) on the primary branch) becomes:

$$\begin{cases} -\frac{1}{\tau_E}\left(\mu_E^{(0)}+\frac{\mu_E^{(1)}}{x^2}\right)+\frac{N_E-1}{N-1}J_{EE}\left[\mathscr{A}_E\left(\mu_E^{(0)}\right)+\mathscr{A}_E'\left(\mu_E^{(0)}\right)\frac{\mu_E^{(1)}}{x^2}\right]+\frac{N_I}{N-1}J_{EI}\nu_I^{\max}\left(1-\frac{1}{4x^2}\right)+I_E=0 \\ -\frac{1}{\tau_I}\left(\frac{2x}{\Lambda_I}+V_I^T\right)+\frac{N_I-1}{N-1}J_{II}\nu_I^{\max}\left(1-\frac{1}{4x^2}\right)+\frac{N_E}{N-1}J_{IE}\left[\mathscr{A}_E\left(\mu_E^{(0)}\right)+\mathscr{A}_E'\left(\mu_E^{(0)}\right)\frac{\mu_E^{(1)}}{x^2}\right]+I_I=0 \end{cases} \tag{S2}$$

Now in the first equation of (S2) we compare all the coefficients with the same perturbative order $\frac{1}{x^{2n}}$, obtaining:

$$-\frac{1}{\tau_E}\mu_E^{(0)}+\frac{N_E-1}{N-1}J_{EE}\mathscr{A}_E\left(\mu_E^{(0)}\right)+\frac{N_I}{N-1}J_{EI}\nu_I^{\max}+I_E=0 \tag{S3}$$

for $n=0$, and:

$$-\frac{1}{\tau_E}\mu_E^{(1)}+\frac{N_E-1}{N-1}J_{EE}\mathscr{A}_E'\left(\mu_E^{(0)}\right)\mu_E^{(1)}-\frac{N_I}{N-1}J_{EI}\frac{\nu_I^{\max}}{4}=0 \tag{S4}$$

for $n=1$. Remembering that $\mathscr{A}_E\left(\mu_E\right)$ is given by (S1), Eq. (S3) can be transformed into a fourth-order polynomial equation:

$$\overline{a}\left(\mu_E^{(0)}\right)^4+\overline{b}\left(\mu_E^{(0)}\right)^3+\overline{c}\left(\mu_E^{(0)}\right)^2+\overline{d}\mu_E^{(0)}+\overline{e}=0 \tag{S5}$$

where:

$$
\begin{aligned}
\overline{a} =& \frac{\Lambda_E^2}{4\tau_E^2} \\
\overline{b} =& -\frac{\Lambda_E^2}{2\tau_E}\left(\overline{\psi} + \frac{V_E^T}{\tau_E}\right) \\
\overline{c} =& \frac{\Lambda_E^2}{4}\left[\overline{\psi}^2 + \left(\frac{V_E^T}{\tau_E}\right)^2 + \frac{4}{\tau_E}V_E^T\overline{\psi}\right] + \frac{1}{\tau_E^2} - \overline{\xi} \\
\overline{d} =& -\frac{\Lambda_E^2}{2}\overline{\psi}V_E^T\left(\frac{V_E^T}{\tau_E} + \overline{\psi}\right) - \frac{2}{\tau_E}\overline{\psi} + 2\overline{\xi}V_E^T \\
\overline{e} =& \left(\frac{\Lambda_E}{2}\overline{\psi}V_E^T\right)^2 + \overline{\psi}^2 - \overline{\xi}\left(V_E^T\right)^2 \\
\overline{\psi} =& \frac{N_E - 1}{N - 1}J_{EE}\frac{\nu_E^{\max}}{2} + \frac{N_I}{N-1}J_{EI}\nu_I^{\max} + I_E \\
\overline{\xi} =& \left(\frac{N_E - 1}{N - 1}J_{EE}\frac{\nu_E^{\max}\Lambda_E}{4}\right)^2
\end{aligned}
\tag{S6}
$$

The solutions of Eq. (S5) are:

$$
\begin{aligned}
\left[\mu_E^{(0)}\right]_{0,1} =& -\frac{\overline{b}}{4\overline{a}} - \overline{Z} \pm \frac{1}{2}\sqrt{-4\overline{Z}^2 - 2\overline{p} + \frac{\overline{q}}{\overline{Z}}} \\
\left[\mu_E^{(0)}\right]_{2,3} =& -\frac{\overline{b}}{4\overline{a}} + \overline{Z} \pm \frac{1}{2}\sqrt{-4\overline{Z}^2 - 2\overline{p} - \frac{\overline{q}}{\overline{Z}}}
\end{aligned}
\tag{S7}
$$

where:

$$
\begin{aligned}
\overline{p} =& \frac{8\overline{a}\overline{c} - 3\overline{b}^2}{8\overline{a}^2} \\
\overline{q} =& \frac{\overline{b}^3 - 4\overline{a}\overline{b}\overline{c} + 8\overline{a}^2\overline{d}}{8\overline{a}^3} \\
\overline{Z} =& \frac{1}{2}\sqrt{-\frac{2}{3}\overline{p} + \frac{1}{3\overline{a}}\left(\overline{Q} + \frac{\overline{\Delta}_0}{\overline{Q}}\right)} \\
\overline{Q} =& \sqrt[3]{\frac{\overline{\Delta}_1 + \sqrt{\overline{\Delta}_1^2 - 4\overline{\Delta}_0^3}}{2}} \\
\overline{\Delta}_0 =& \overline{c}^2 - 3\overline{b}\overline{d} + 12\overline{a}\overline{e} \\
\overline{\Delta}_1 =& 2\overline{c}^3 - 9\overline{b}\overline{c}\overline{d} + 27\overline{b}^2\overline{e} + 27\overline{a}\overline{d}^2 - 72\overline{a}\overline{c}\overline{e}
\end{aligned}
\tag{S8}
$$

Clearly, some solutions $\mu_E^{(0)}$ may be complex and must be discarded, since we want to describe stationary membrane potentials, which are real quantities. On the other side, from Eq. (S4) we obtain:

$$
\mu_E^{(1)} = \frac{\frac{N_I}{N-1} J_{EI} \frac{\nu_I^{\max}}{4}}{-\frac{1}{\tau_E} + \frac{N_E - 1}{N-1} J_{EE} \mathscr{A}_E' \left(\mu_E^{(0)}\right)} \tag{S9}
$$

The second equation of (S2) contains a term proportional to $x$. For this reason it cannot be solved as the first equation of (S2) (namely by comparing all the terms with the same order $\frac{1}{x^{2n}}$), so we have to solve it directly without further simplifications. We observe that it can be transformed into the following third-order polynomial equation:

$$
\widetilde{a}x^3 + \widetilde{b}x^2 + \widetilde{c}x + \widetilde{d} = 0
$$

where:

$$
\begin{aligned}
\widetilde{a} =& \frac{2}{\Lambda_I \tau_I} \\
\widetilde{b} =& -\left(\frac{N_I - 1}{N-1} J_{II} \nu_I^{\max} + \frac{N_E}{N-1} J_{IE} \mathscr{A}_E \left(\mu_E^{(0)}\right) + I_I - \frac{V_I^T}{\tau_I}\right) \\
\widetilde{c} =& 0 \\
\widetilde{d} =& \frac{N_I - 1}{N-1} J_{II} \frac{\nu_I^{\max}}{4} - \frac{N_E}{N-1} J_{IE} \mathscr{A}_E' \left(\mu_E^{(0)}\right) \mu_E^{(1)}
\end{aligned}
\tag{S10}
$$

Its solutions are:

$$x_k = -\frac{1}{3\widetilde{a}}\left(\widetilde{b} + u_k\widetilde{Q} + \frac{\widetilde{\Delta}_0}{u_k\widetilde{Q}}\right) \tag{S11}$$

for $k = 0, 1, 2$, where:

$$u_0 = 1, \qquad u_1 = \tfrac{-1+\iota\sqrt{3}}{2}, \qquad u_2 = \tfrac{-1-\iota\sqrt{3}}{2}$$

$$\begin{aligned}
\widetilde{Q} =& \sqrt[3]{\frac{\widetilde{\Delta}_1 + \sqrt{\widetilde{\Delta}_1^2 - 4\widetilde{\Delta}_0^3}}{2}} \\
\widetilde{\Delta}_0 =& \widetilde{b}^2 \\
\widetilde{\Delta}_1 =& 2\widetilde{b}^3 + 27\widetilde{a}^2\widetilde{d}
\end{aligned}$$

and $\iota = \sqrt{-1}$. According to the De Moivre's formula, for every $u_k$ we have different solutions of the square and cube roots that define $\widetilde{Q}$. Different combinations of $\mu_E^{(0)}$, $u_k$ and De Moivre's solutions provide equivalent results for $x$. So after removing all the redundant and complex solutions, we obtain only 3 or 5 possible formulas for $\widetilde{Q}$, depending on the strength of $I_I$.

We start by analyzing the case with weak inhibitory current, e.g. $I_I = -10$. If we choose for example $u_2$, we get 5 solutions:

$$\widetilde{Q}_{\mathrm{green}} = \tfrac{1}{2}\sqrt[3]{\tfrac{\left|\widetilde{\Delta}_1 + \sqrt{\widetilde{\Delta}_1^2 - 4\widetilde{\Delta}_0^3}\right|}{2}}\left(1 - \iota\sqrt{3}\right), \qquad \mu_E^{(0)} = \left[\mu_E^{(0)}\right]_2, \qquad \widetilde{\Delta}_1^2 - 4\widetilde{\Delta}_0^3 \geq 0$$

$$\left.\begin{aligned}
\widetilde{Q}_{\mathrm{yellow,\,blue}} &= \sqrt{\widetilde{\Delta}_0}\left(\cos\vartheta - \iota\sin\vartheta\right), \qquad \mu_E^{(0)} = \left[\mu_E^{(0)}\right]_{3,0} \\
\widetilde{Q}_{\mathrm{red,\,cyan}} &= \sqrt{\widetilde{\Delta}_0}\left(\cos\vartheta + \iota\sin\vartheta\right), \qquad \mu_E^{(0)} = \left[\mu_E^{(0)}\right]_{0,3}
\end{aligned}\right\} \widetilde{\Delta}_0 \geq 0,\ \vartheta = \frac{1}{3}\mathrm{atan2}\left(\sqrt{4\widetilde{\Delta}_0^3 - \widetilde{\Delta}_1^2}, \widetilde{\Delta}_1\right),\ 4\widetilde{\Delta}_0^3 - \widetilde{\Delta}_1^2 \geq 0$$

where the colors refer to those of the top panels in Fig. (S1). So from Eq. (S11) we obtain:

$$
\begin{aligned}
x_{\text{green}} &= -\frac{1}{3\widetilde{a}}\left(\widetilde{b}-\sqrt[3]{\frac{\left|\widetilde{\Delta}_1+\sqrt{\widetilde{\Delta}_1^2-4\widetilde{\Delta}_0^3}\right|}{2}}-\frac{\widetilde{b}^2}{\sqrt[3]{\frac{\left|\widetilde{\Delta}_1+\sqrt{\widetilde{\Delta}_1^2-4\widetilde{\Delta}_0^3}\right|}{2}}}\right), \qquad \mu_E^{(0)} = \left[\mu_E^{(0)}\right]_2 \\
x_{\text{yellow, blue}} &= -\frac{\widetilde{b}}{3\widetilde{a}}\left(1+\sqrt{3}\sin\vartheta+\cos\vartheta\right), \qquad \mu_E^{(0)} = \left[\mu_E^{(0)}\right]_{3,0} \\
x_{\text{red, cyan}} &= -\frac{\widetilde{b}}{3\widetilde{a}}\left(1-\sqrt{3}\sin\vartheta+\cos\vartheta\right), \qquad \mu_E^{(0)} = \left[\mu_E^{(0)}\right]_{0,3}
\end{aligned}
\tag{S12}
$$

Finally, from the formulas $\mu_E = \mu_E^{(0)} + \frac{\mu_E^{(1)}}{x^2}$ and $\mu_I = \frac{2x}{\Lambda_I} + V_I^T$ we get the membrane potentials in the two populations, as shown in the top panels of Fig. (S1). From this figure, on all the portions of the curve we observe a good agreement between the analytical formulas and the numerical solutions provided by Cl_MatCont, with the exception of most of the cyan colored curve, and also the green and yellow ones close to point $A$.

Now we have to find the coordinates of the points $A$, $B$, $C$, $D$ that define the ranges of our 5 colored portions of the primary branch. Clearly the most interesting ones are the points $A$, $C$ since there the system undergoes a saddle-node bifurcation (LP for short). At point $A$, the zeroth-order approximation is very precise (i.e. $\mu_E(A) \approx \mu_E^{(0)}(A)$) since $\mu_I(A) \gg 1$, so we can use it to find the coordinates of this bifurcation point. If we take the derivative with respect to $\mu_E^{(0)}$ of Eq. (S3), we obtain:

$$
\frac{dI_E}{d\mu_E^{(0)}} = \frac{1}{\tau_E} - \frac{N_E-1}{N-1} J_{EE} \mathscr{A}_E' \left(\mu_E^{(0)}\right) \tag{S13}
$$

where, according to Eq. (S1):

$$
\mathscr{A}_\alpha'(V) = \frac{\nu_\alpha^{\max}\Lambda_\alpha}{4} \frac{1}{\sqrt{\left[1+\frac{\Lambda_\alpha^2}{4}\left(V-V_\alpha^T\right)^2\right]^3}} \tag{S14}
$$

Since $\frac{dI_E}{d\mu_E^{(0)}} = 0$ at point $A$, we obtain:

$$
\mu_E^{(0)}(A) = V_E^T + \frac{2}{\Lambda_E}\sqrt{\sqrt[3]{\left(\frac{N_E-1}{N-1}J_{EE}\frac{\nu_E^{\max}\Lambda_E}{4}\tau_E\right)^2}-1} \tag{S15}
$$

We discard the solution with the $-\sqrt{\ }$, because it is quantitatively different from the numerical value of $\mu_E(A)$ provided by Cl_MatCont (its meaning will be clarified later in this section). Now, if we replace Eq. (S15) into Eq. (S3), we get:

$$
I_E(A) = \frac{1}{\tau_E}\mu_E^{(0)}(A) - \frac{N_E-1}{N-1}J_{EE}\mathscr{A}_E\left(\mu_E^{(0)}(A)\right) - \frac{N_I}{N-1}J_{EI}\nu_I^{\max} \tag{S16}
$$

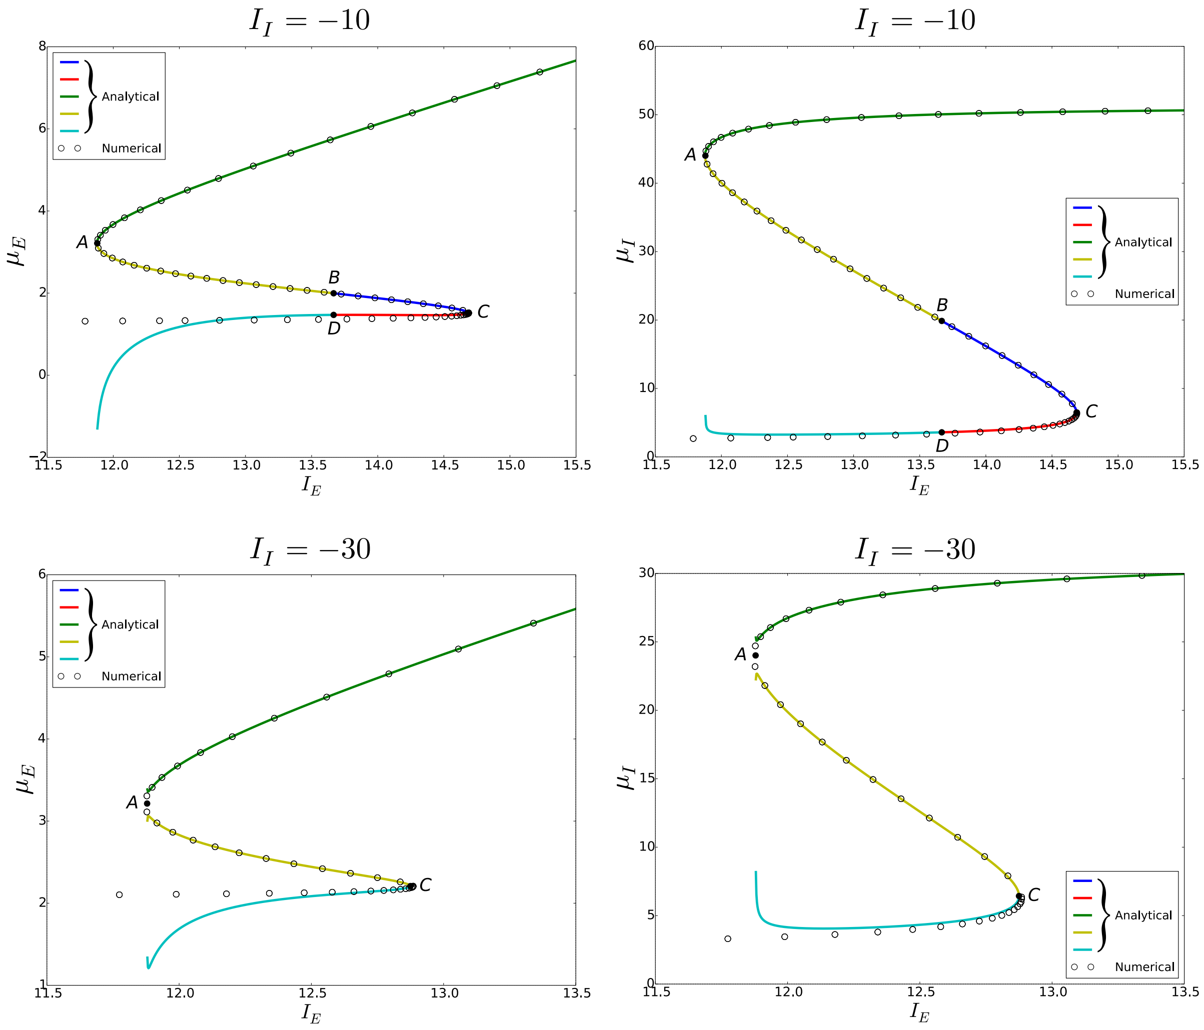


Figure S1: Equilibrium points obtained from the first-order perturbative expansion of the system (5) or (10) on the primary branch. The panels on the top represent the solutions $\mu_{E,I}$ for $I_I = -10$, while those at the bottom are the solutions for $I_I = -30$. The figure shows a good agreement with the numerical solutions provided by Cl_MatCont on all the portions of the primary branch with the exception of most of the cyan colored curve, and also the green and yellow ones close to point $A$, where the first-order perturbative approximation does not work anymore due to the divergence of $\mu_E^{(1)}$. For $I_I = -10$ the curves $\mu_{E,I}$ are made of 5 portions (green, yellow, blue, red, cyan), while for $I_I = -30$ the blue and red branches disappear, see text.

From Eq. (S13) we see that the first-order correction does not work around $A$, because the right-hand side of this formula is equal to zero in $A$. This term is also the denominator of $\mu_E^{(1)}$ (see Eq. (S9)), which explains why in $A$ the first-order correction cannot be applied. Nevertheless, here the zeroth-order approximation (S15) + (S16) is in very good agreement with the numerical equilibrium points.

To conclude, from the second equation of (5) or (10), we get:

$$-\frac{1}{\tau_I}\mu_I(A) + \frac{N_I - 1}{N-1} J_{II} \mathscr{A}_I(\mu_I(A)) + \frac{N_E}{N-1} J_{IE} \mathscr{A}_E\left(\mu_E^{(0)}(A)\right) + I_I = 0 \tag{S17}$$

Since $\mu_I(A) \gg 1$ and therefore $\mathscr{A}_I(\mu_I(A)) \approx \nu_I^{\max}$, we obtain:

$$\mu_I(A) \approx \tau_I \left(\frac{N_I - 1}{N-1} J_{II} \nu_I^{\max} + \frac{N_E}{N-1} J_{IE} \mathscr{A}_E\left(\mu_E^{(0)}(A)\right) + I_I\right)$$

A more precise way to calculate $\mu_I(A)$ is to solve directly Eq. (S17), which can be transformed into the following fourth-order polynomial equation:

$$\breve{a}\mu_I^4(A) + \breve{b}\mu_I^3(A) + \breve{c}\mu_I^2(A) + \breve{d}\mu_I(A) + \breve{e} = 0 \tag{S18}$$

where:

$$\begin{aligned}
\breve{a} &= \frac{\Lambda_I^2}{4\tau_I^2} \\
\breve{b} &= -\frac{\Lambda_I^2}{2\tau_I}\left(\breve{\psi} + \frac{V_I^T}{\tau_I}\right) \\
\breve{c} &= \frac{\Lambda_I^2}{4}\left[\breve{\psi}^2 + \left(\frac{V_I^T}{\tau_I}\right)^2 + \frac{4}{\tau_I} V_I^T \breve{\psi}\right] + \frac{1}{\tau_I^2} - \breve{\xi} \\
\breve{d} &= -\frac{\Lambda_I^2}{2}\breve{\psi} V_I^T \left(\frac{V_I^T}{\tau_I} + \breve{\psi}\right) - \frac{2}{\tau_I}\breve{\psi} + 2\breve{\xi} V_I^T \\
\breve{e} &= \left(\frac{\Lambda_I}{2}\breve{\psi} V_I^T\right)^2 + \breve{\psi}^2 - \breve{\xi}\left(V_I^T\right)^2 \\
\breve{\psi} &= \frac{N_I - 1}{N-1} J_{II} \frac{\nu_I^{\max}}{2} + \frac{N_E}{N-1} J_{IE} \mathscr{A}_E\left(\mu_E^{(0)}(A)\right) + I_I \\
\breve{\xi} &= \left(\frac{N_I - 1}{N-1} J_{II} \frac{\nu_I^{\max}\Lambda_I}{4}\right)^2
\end{aligned}$$

The solutions of Eq. (S18) are:

$$[\mu_I(A)]_{0,1} = -\frac{\breve{b}}{4\breve{a}} - \breve{Z} \pm \frac{1}{2}\sqrt{-4\breve{Z}^2 - 2\breve{p} + \frac{\breve{q}}{\breve{Z}}}$$

$$[\mu_I(A)]_{2,3} = -\frac{\breve{b}}{4\breve{a}} + \breve{Z} \pm \frac{1}{2}\sqrt{-4\breve{Z}^2 - 2\breve{p} - \frac{\breve{q}}{\breve{Z}}}$$

where $\breve{Z}$, $\breve{p}$, $\breve{q}$ are defined similarly to Eq. (S8). It is easy to check that the solution that represents the membrane potential in $A$ is $[\mu_I(A)]_3 = -\frac{\breve{b}}{4\breve{a}} + \breve{Z} - \frac{1}{2}\sqrt{-4\breve{Z}^2 - 2\breve{p} - \frac{\breve{q}}{\breve{Z}}}$, because $[\mu_I(A)]_{0,1,2}$ are quantitatively different from the numerical value of $\mu_I(A)$ provided by Cl_MatCont.

Things are more complicated for the point $C$. In this case we have to use the whole theory with the first-order correction, because the zeroth-order approximation is not able to describe this bifurcation point. Since $C$ is the connection point between the blue and red portions of the primary branch (see Fig. (S1), top), it can be defined through the relation $x_{\text{red}} = x_{\text{blue}}$. So, from Eq. (S12) we can see that this relation is equivalent to $\vartheta = 0$, namely $4\widetilde{\Delta}_0^3 - \widetilde{\Delta}_1^2 = 0$. From the expressions of $\widetilde{\Delta}_0$ and $\widetilde{\Delta}_1$ we obtain that this equation can be rewritten as $27\widetilde{a}^2\widetilde{d}\left(4\widetilde{b}^3 + 27\widetilde{a}^2\widetilde{d}\right) = 0$. Now it is possible to prove that $\widetilde{d} \neq 0$ at point $C$, therefore the final equation that describes this bifurcation point is:

$$4\widetilde{b}^3 + 27\widetilde{a}^2\widetilde{d} = 0 \tag{S19}$$

However, Eq. (S19) cannot be solved exactly, so we use it to calculate numerically $\mu_E^{(0)}(C)$, which in turn allows us to get $\mu_E^{(1)}(C)$ from Eq. (S9). Moreover, from the condition $\vartheta = 0$ we know that $x = -\frac{2\widetilde{b}}{3\widetilde{a}}$ (see Eq. (S12)), and finally we calculate $\mu_E(C)$ through $\mu_E = \mu_E^{(0)} + \frac{\mu_E^{(1)}}{x^2}$, $\mu_I(C)$ from $\mu_I = \frac{2x}{\Lambda_I} + V_I^T$, and $I_E(C)$ by means of Eq. (S3), similarly to point $A$ (see Eq. (S16)).

Now we consider the point $B$. Since this is the connection point between the yellow and blue portions of the primary branch, it has to satisfy the condition $x_{\text{yellow}} = x_{\text{blue}}$, so from Eq. (S12) we get that this is equivalent to $\left[\mu_E^{(0)}\right]_3 = \left[\mu_E^{(0)}\right]_0$. The last condition is satisfied at the inflection point of the curve $\mu_E^{(0)} = \mu_E^{(0)}(I_E)$, so the point $B$ can be calculated from the equation $\frac{d^2 I_E}{d\left[\mu_E^{(0)}\right]^2} = 0$. Now, from Eq. (S13) we get:

$$\frac{d^2 I_E}{d\left[\mu_E^{(0)}\right]^2} = -\frac{N_E - 1}{N - 1} J_{EE} \mathscr{A}_E''\left(\mu_E^{(0)}\right) \tag{S20}$$

Since:

$$\mathscr{A}_\alpha''(V) = -\frac{3\nu_\alpha^{\max}\Lambda_\alpha^3}{16}\frac{V - V_\alpha^T}{\sqrt{\left[1 + \frac{\Lambda_\alpha^2}{4}\left(V - V_\alpha^T\right)^2\right]^5}} \tag{S21}$$

we conclude that $\mu_E^{(0)}(B) = V_E^T$, or in other terms $\left[\mu_E^{(0)}\right]_3 = \left[\mu_E^{(0)}\right]_0 = V_E^T$ in $B$. Similarly to point $C$, we can use $\mu_E^{(0)}(B)$ to calculate $\mu_E^{(1)}(B)$ and $x$ (we can use $x_{\text{yellow}}$ or equivalently $x_{\text{blue}}$), from which we get $\mu_E(B)$, $\mu_I(B)$ and $I_E(B)$. The same idea can be applied to calculate the coordinates of the point $D$, since again $x_{\text{red}} = x_{\text{cyan}}$ when $\left[\mu_E^{(0)}\right]_0 = \left[\mu_E^{(0)}\right]_3$. The only difference with point $B$ is that now the variable $x$ must be calculated through the formula of $x_{\text{red}}$ or that of $x_{\text{cyan}}$. Clearly we also get $I_E(D) = I_E(B) = \frac{1}{\tau_E}V_E^T - \frac{N_E-1}{N-1}J_{EE}\frac{\nu_E^{\max}}{2} - \frac{N_I}{N-1}J_{EI}\nu_I^{\max}$, which is in agreement with Fig. (S1).

On the other side, when $I_I$ is sufficiently large and negative, e.g. $I_I = -30$, the term $\widetilde{\Delta}_1^2 - 4\widetilde{\Delta}_0^3$ can be zero on the yellow and cyan portions for some $I_E < I_E(B)$. At this point $\vartheta = 0$, so according to Eq. (S12), we get $x_{\text{yellow}} = x_{\text{cyan}}$, or in other terms the two portions meet each other. In this way the point $C$ is formed by the yellow and cyan portions, while the blue and red ones disappear from the primary branch (see Fig. (S1), bottom).

In general we observe that the divergence of the perturbative expansion on the cyan portion of the primary branch around point $A$ prevents the use of our approximation for studying the secondary branches that emanate from the branching point. This is due to the fact that these branches extend to $I_E < I_E(A)$ (see Figs. (8) and (9)), where the perturbative approximation cannot be used anymore, because the membrane potential $\mu_I(A)$ is not large enough to saturate the activation function. We also observe that, according to the numerical analysis performed in [1], for $I_E \ll I_E(A)$ we can have other LP bifurcations. As we said at the beginning of this section, the term $\mathscr{A}_I(\mu_I)$ in Eqs. (5) or (10) saturates to 0 or $\nu_I^{\max}$. Up to now we have considered the case $\mathscr{A}_I(\mu_I) \approx \nu_I^{\max}$, while the remaining LP bifurcations are obtained when the activation function saturates to zero. In this case we have to use the following asymptotic expansion for $\mu_I \to -\infty$:

$$\mathscr{A}_I(\mu_I) \approx \frac{\nu_I^{\max}}{4x^2} \tag{S22}$$

We do not show the explicit calculation of the equilibrium points, which is left to the interested readers.

Clearly our approximation can be improved if we consider higher orders in the perturbative expansion. At the second order we get $\mu_E = \mu_E^{(0)} + \frac{\mu_E^{(1)}}{x^2} + \frac{\mu_E^{(2)}}{x^4}$, which means that when $\mathscr{A}_I(\mu_I)$ saturates for example to $\nu_I^{\max}$, we have to use the asymptotic expansion $\mathscr{A}(\mu_I) \approx \nu_I^{\max}\left(1 - \frac{1}{4x^2} + \frac{3}{16x^4}\right)$ for $\mu_I \to +\infty$. In this case, the variable $x$ satisfies a fifth-order polynomial equation, which can be solved analytically in terms of complicated Jacobi theta functions [2]. However also in this case the the formulas of $\mu_{E,I}$ diverge for $I_E \to I_E(A)$, due to explosion of both the terms $\mu_E^{(1)}$ and $\mu_E^{(2)}$. This justifies the use of the first-order approximation developed in this section, by virtue of its lower complexity.

# S3 Weak-inhibition regime

In this section we perform an analytical study of the bifurcations in the weak-inhibition regime. In more detail, in SubSec. (S3.1) we find the analytical formulas of the eigenvalues of the neural network, which will be used to derive its analytical codimension two bifurcation diagram, as shown in SubSec. (S3.2).

## S3.1 Eigenvalues

As we said in [1], for weak inhibition the membrane potentials are homogeneous in each population, therefore it is easy to verify that in this case the Jacobian matrix $\mathcal{J}$ of the network at the equilibrium points is:

$$\mathcal{J}=\left[\begin{array}{cc}\mathscr{J}_{EE} & \mathscr{J}_{EI}\\ \mathscr{J}_{IE} & \mathscr{J}_{II}\end{array}\right],\qquad \mathscr{J}_{\alpha\beta}=\begin{cases}-\frac{1}{\tau_\alpha}\mathrm{Id}_{N_\alpha}+\frac{J_{\alpha\alpha}}{N-1}\mathscr{A}'_\alpha\left(\mu_\alpha\right)\left(\mathbb{I}_{N_\alpha}-\mathrm{Id}_{N_\alpha}\right), & \text{for } \alpha=\beta\\ \\ \frac{J_{\alpha\beta}}{N-1}\mathscr{A}'_\beta\left(\mu_\beta\right)\mathbb{I}_{N_\alpha,N_\beta}, & \text{for } \alpha\neq\beta\end{cases} \tag{S23}$$

where $\mu_\alpha$ are the solutions of Eq. (5), $\mathbb{I}_{N_\alpha,N_\beta}$ is the $N_\alpha \times N_\beta$ all-ones matrix (with $\mathbb{I}_{N_\alpha} \stackrel{\text{def}}{=} \mathbb{I}_{N_\alpha,N_\alpha}$), and $\mathrm{Id}_{N_\alpha}$ is the $N_\alpha \times N_\alpha$ identity matrix. The characteristic equation of the system is $\det\left(\mathcal{J}-\lambda\mathrm{Id}_N\right)=0$, where $\lambda$ are the eigenvalues of the Jacobian matrix. In other terms, the equation that we need to solve is:

$$\det\left(\left[\begin{array}{cc}\mathscr{J}_{EE}-\lambda\mathrm{Id}_{N_E} & \mathscr{J}_{EI}\\ \mathscr{J}_{IE} & \mathscr{J}_{II}-\lambda\mathrm{Id}_{N_I}\end{array}\right]\right)=0 \tag{S24}$$

We can evaluate this determinant by means of the following formulas for block matrices:

$$\det\left(\left[\begin{array}{cc}\mathfrak{A} & \mathfrak{B}\\ \mathfrak{C} & \mathfrak{D}\end{array}\right]\right)=\begin{cases}\det\left(\mathfrak{A}\right)\det\left(\mathfrak{D}-\mathfrak{C}\mathfrak{A}^{-1}\mathfrak{B}\right), \text{ if } \det\left(\mathfrak{A}\right)\neq 0\\ \\ \det\left(\mathfrak{D}\right)\det\left(\mathfrak{A}-\mathfrak{B}\mathfrak{D}^{-1}\mathfrak{C}\right), \text{ if } \det\left(\mathfrak{D}\right)\neq 0\end{cases} \tag{S25}$$

where in our case $\mathfrak{A}=\mathscr{J}_{EE}-\lambda\mathrm{Id}_{N_E}$, $\mathfrak{B}=\mathscr{J}_{EI}$, $\mathfrak{C}=\mathscr{J}_{IE}$, $\mathfrak{D}=\mathscr{J}_{II}-\lambda\mathrm{Id}_{N_I}$.

We start by calculating the eigenvalues $\lambda_i$ of $\mathcal{J}$ such that $\det\left(\mathscr{J}_{II}-\lambda_i\mathrm{Id}_{N_I}\right)\neq 0$ for some values of the index $i$. In other terms, we start by finding the eigenvalues of $\mathcal{J}$ which are not also eigenvalues of $\mathscr{J}_{II}$, if they exist. Therefore we have to suppose that $\lambda_i \neq \lambda_j^{II}$ for $j=0,\ldots,N_I-1$, where $\lambda_j^{II}$ are the eigenvalues of $\mathscr{J}_{II}$:

$$\lambda_0^{II}=-\frac{1}{\tau_I}+\frac{N_I-1}{N-1}J_{II}\mathscr{A}'_I\left(\mu_I\right)$$

$$\lambda_j^{II}=-\left[\frac{1}{\tau_I}+\frac{J_{II}}{N-1}\mathscr{A}'_I\left(\mu_I\right)\right],\qquad j=1,\ldots,N_I-1$$

By using the second formula in Eq. (S25), we get that Eq. (S24) implies:

$$\det\left(\mathfrak{A}-\mathfrak{B}\mathfrak{D}^{-1}\mathfrak{C}\right)=0 \tag{S26}$$

Now, since $\mathfrak{D}$ is a circulant matrix:

$$\mathfrak{D}=\mathfrak{d}_0\mathrm{Id}_{N_I}+\mathfrak{d}_1\left(\mathbb{I}_{N_I}-\mathrm{Id}_{N_I}\right),\quad \mathfrak{d}_0=-\frac{1}{\tau_I}-\lambda_i,\quad \mathfrak{d}_1=\frac{J_{II}}{N-1}\mathscr{A}'_I\left(\mu_I\right)$$

then $\mathfrak{D}^{-1}$ is also circulant:

$$\mathfrak{D}^{-1} = \mathfrak{m}_0 \mathrm{Id}_{N_I} + \mathfrak{m}_1 \left(\mathbb{I}_{N_I} - \mathrm{Id}_{N_I}\right), \quad \mathfrak{m}_0 = \frac{1 - \frac{\mathfrak{d}_1 (N_I - 1)}{\mathfrak{d}_1 - \mathfrak{d}_0}}{\mathfrak{d}_0 + \mathfrak{d}_1 (N_I - 1)}, \quad \mathfrak{m}_1 = \mathfrak{m}_0 + \frac{1}{\mathfrak{d}_1 - \mathfrak{d}_0}$$

where the denominators in $\mathfrak{m}_{0,1}$ cannot be equal to zero due to the hypothesis $\lambda_i \neq \lambda_j^{II}$. Now, due to the properties of the circulant matrices, $\mathfrak{A} - \mathfrak{B}\mathfrak{D}^{-1}\mathfrak{C}$ is circulant as well:

$$\mathfrak{A} - \mathfrak{B}\mathfrak{D}^{-1}\mathfrak{C} = \mathfrak{n}_0 \mathrm{Id}_{N_E} + \mathfrak{n}_1 \left(\mathbb{I}_{N_E} - \mathrm{Id}_{N_E}\right)$$

$$\mathfrak{n}_0 = \mathfrak{a}_0 - \mathfrak{r}, \quad \mathfrak{n}_1 = \mathfrak{a}_1 - \mathfrak{r}, \quad \mathfrak{r} = N_I \mathfrak{b}_0 \mathfrak{c}_0 \left[\mathfrak{m}_0 + (N_I - 1)\, \mathfrak{m}_1\right]$$

$$\mathfrak{a}_0 = -\frac{1}{\tau_E} - \lambda_i, \quad \mathfrak{a}_1 = \frac{J_{EE}}{N-1} \mathscr{A}_E' (\mu_E), \quad \mathfrak{b}_0 = \frac{J_{EI}}{N-1} \mathscr{A}_I' (\mu_I), \quad \mathfrak{c}_0 = \frac{J_{IE}}{N-1} \mathscr{A}_E' (\mu_E)$$

So its determinant is:

$$\det\left(\mathfrak{A} - \mathfrak{B}\mathfrak{D}^{-1}\mathfrak{C}\right) = \prod_{j=0}^{N_E - 1} \left(\mathfrak{n}_0 + \mathfrak{n}_1 \sum_{k=1}^{N_E - 1} e^{\frac{2\pi j k}{N_E} \iota}\right) = \prod_{j=0}^{N_E - 1} \left[\mathfrak{n}_0 + \mathfrak{n}_1 \left(\frac{1 - e^{2\pi j \iota}}{1 - e^{\frac{2\pi j}{N_E} \iota}} - 1\right)\right]$$

$$= \left[\mathfrak{n}_0 + \mathfrak{n}_1 (N_E - 1)\right] (\mathfrak{n}_0 - \mathfrak{n}_1)^{N_E - 1}$$

Therefore the characteristic equation (S26) gives:

$$\mathfrak{n}_0 + \mathfrak{n}_1 (N_E - 1) = 0 \qquad \text{and/or} \qquad \mathfrak{n}_0 - \mathfrak{n}_1 = 0 \tag{S27}$$

Now we start to analyze the first equation of (S27). From it we obtain:

$$\mathfrak{a}_0 - \mathfrak{r} + (\mathfrak{a}_1 - \mathfrak{r}) (N_E - 1) = 0$$

and therefore, by substitution:

$$-\lambda_i - \gamma \left(N_I \frac{1 - \frac{\varepsilon}{\lambda_i + \zeta}}{-\lambda_i + \eta} + \frac{N_I - 1}{\lambda_i + \zeta}\right) + \delta = 0 \tag{S28}$$

where:

$$\gamma = \frac{N_E N_I}{(N-1)^2} J_{EI} J_{IE} \mathscr{A}_E' (\mu_E) \mathscr{A}_I' (\mu_I), \quad \delta = -\frac{1}{\tau_E} + \frac{N_E - 1}{N-1} J_{EE} \mathscr{A}_E' (\mu_E)$$

$$\varepsilon = \frac{N_I - 1}{N-1} J_{II} \mathscr{A}_I' (\mu_I), \quad \zeta = \frac{1}{\tau_I} + \frac{J_{II}}{N-1} \mathscr{A}_I' (\mu_I), \quad \eta = -\frac{1}{\tau_I} + \frac{N_I - 1}{N-1} J_{II} \mathscr{A}_I' (\mu_I) \tag{S29}$$

Now, since:

$$N_I \frac{1 - \frac{\varepsilon}{\lambda_i + \zeta}}{-\lambda_i + \eta} + \frac{N_I - 1}{\lambda_i + \zeta} = \frac{1}{-\lambda_i + \eta}$$

Eq. (S28) can be rewritten as the following polynomial equation:

$$\lambda_i^2 - (\delta + \eta) \lambda_i + (\delta\eta - \gamma) = 0 \tag{S30}$$

whose solutions are:

$$\lambda_{0,1} = \frac{\delta + \eta \pm \sqrt{(\delta + \eta)^2 - 4(\delta\eta - \gamma)}}{2}$$

According to the sign of the discriminant $\Delta = (\delta + \eta)^2 - 4(\delta\eta - \gamma) = (\delta - \eta)^2 + 4\gamma$, the eigenvalues $\lambda_{0,1}$ can be real and distinct ($\Delta > 0$), real and identical ($\Delta = 0$), or complex conjugated ($\Delta < 0$).

Now we consider the second equation of (S27). From it we obtain $\mathfrak{a}_0 = \mathfrak{a}_1$ and therefore:

$$\lambda_i = -\left[\frac{1}{\tau_E} + \frac{J_{EE}}{N-1} \mathscr{A}_E' (\mu_E)\right], \qquad i = 2, \ldots, N_E$$

So we have obtained $N_E - 1$ identical and real eigenvalues, that for simplicity we call $\lambda_E$. However we observe that up to now we have obtained only $N_E + 1$ eigenvalues (considering also $\lambda_{0,1}$), thus some are missing.

To get the remaining eigenvalues, we can repeat the procedure above, but this time we have to calculate the eigenvalues $\lambda_i$ of $\mathcal{J}$ such that $\det(\mathscr{J}_{EE} - \lambda_i \mathrm{Id}_{N_E}) \neq 0$. In this case, by using the first formula in Eq. (S25), we obtain again Eq. (S30), and also the following set of real eigenvalues:

$$\lambda_i = -\left[\frac{1}{\tau_I} + \frac{J_{II}}{N-1} \mathscr{A}_I' (\mu_I)\right], \qquad i = N_E + 1, \ldots, N - 1$$

that we call simply $\lambda_I$.

To sum up, we have obtained that the Jacobian matrix $\mathcal{J}$ at the equilibrium points has the following set of eigenvalues:

$$\lambda_{0,1} = \frac{\delta + \eta \pm \sqrt{(\delta - \eta)^2 + 4\gamma}}{2}, \quad \lambda_E = -\left[\frac{1}{\tau_E} + \frac{J_{EE}}{N-1}\mathscr{A}_E'(\mu_E)\right], \quad \lambda_I = -\left[\frac{1}{\tau_I} + \frac{J_{II}}{N-1}\mathscr{A}_I'(\mu_I)\right] \tag{S31}$$

where $\lambda_{0,1}$ have algebraic multiplicity 1 for $\Delta \neq 0$ or they are identical for $\Delta = 0$, while $\lambda_{E,I}$ have multiplicity $N_{E,I} - 1$. The most fundamental quantity of our theory is the eigenvalue $\lambda_I$, since it determines the formation of the branching point bifurcations discussed in [1].

We conclude by observing that at the beginning of this section we defined qualitatively the weak-inhibition regime by the homogeneity of the membrane potentials. However, the eigenvalue $\lambda_I$ that we have just found allows us to define this regime in a quantitative way. Indeed, as we will explain in the next sections, the membrane potentials in the inhibitory population are always homogeneous if and only if $\lambda_I < 0$, therefore this inequality defines in a rigorous way the weak-inhibition regime. On the other side, when $\lambda_I \geq 0$ the network is in a strong-inhibition regime and it exhibits both homogeneous and heterogeneous solutions, but this will be discussed later in Sec. (S4).

## S3.2 Codimension two bifurcation diagram

In this subsection we derive analytically most of the local bifurcations shown in the weak-inhibition codimension two bifurcation diagram of Fig. (7). In particular, we find a mathematical description of the LP and H curves (SubSecs. (S3.2.1) and (S3.2.2) respectively), as well as the coordinates of the BT points (SubSec. (S3.2.3)), while the CP and GH points are analytically intractable and therefore have to be studied by means of numerical methods.

### S3.2.1 Saddle-node bifurcations on the primary branch

Here we show two different ways to calculate analytically the LP curves of the codimension two bifurcation diagram in Fig. (7) that occur on the primary branch. The first method is based on the results obtained in Sec. (S2) and provides an explicit (i.e. non-parametric) but approximate formula of the LP curves. The idea is to use Eqs. (S16) and (S19), that describe the coordinates of the LP points $A$ and $C$ for a fixed current $I_I$, and to use them to obtain the corresponding curves $I_I = \mathfrak{f}(I_E)$. More explicitly, we can rewrite Eq. (S19) as $\widetilde{b} = -\sqrt[3]{\frac{27}{4}\widetilde{a}^2\widetilde{d}}$, and from the expression of $\widetilde{b}$ shown in Eq. (S10) we can isolate $I_I$ to get:

$$I_I = \frac{V_I^T}{\tau_I} - \frac{N_I - 1}{N-1}J_{II}\nu_I^{\max} - \frac{N_E}{N-1}J_{IE}\mathscr{A}_E\left(\mu_E^{(0)}\right) + \sqrt[3]{\frac{27}{4}\widetilde{a}^2\widetilde{d}} \tag{S32}$$

Now we observe that $\widetilde{a}$ does not depend on the external currents, while $\widetilde{d}$ depends only on $I_E$ through $\mu_E^{(0)}$ (and therefore through the term $\overline{\psi}$, see Eqs. (S7) and (S6)). In this way we obtain $I_I$ as a function of $I_E$. According to the results shown in Sec. (S2), when $I_I$ is large enough (i.e. approximately $I_I > -20$), the point $C$ is generated by the blue and red portions of $\mu_{E,I}$ (see Fig. (S1), top), therefore in this case we have to use $\left[\mu_E^{(0)}\right]_0$ in Eq. (S32). On the contrary, for a strongly negative current (i.e. $I_I < -20$), the point $C$ is generated by the yellow and cyan portions of the primary branch (see Fig. (S1), bottom), therefore in this case we have to use $\left[\mu_E^{(0)}\right]_3$. Through this distinction we get the LP curve shown in Fig. (S2), where the orange and violet portions are obtained in the two regimes of $I_I$ that we have just described. Clearly the point $F$ that separates the two portions occurs when $\left[\mu_E^{(0)}\right]_0 = \left[\mu_E^{(0)}\right]_3$ and therefore at $I_E = I_E(B)$ (so the corresponding $I_I$ can be obtained from Eq. (S32)).

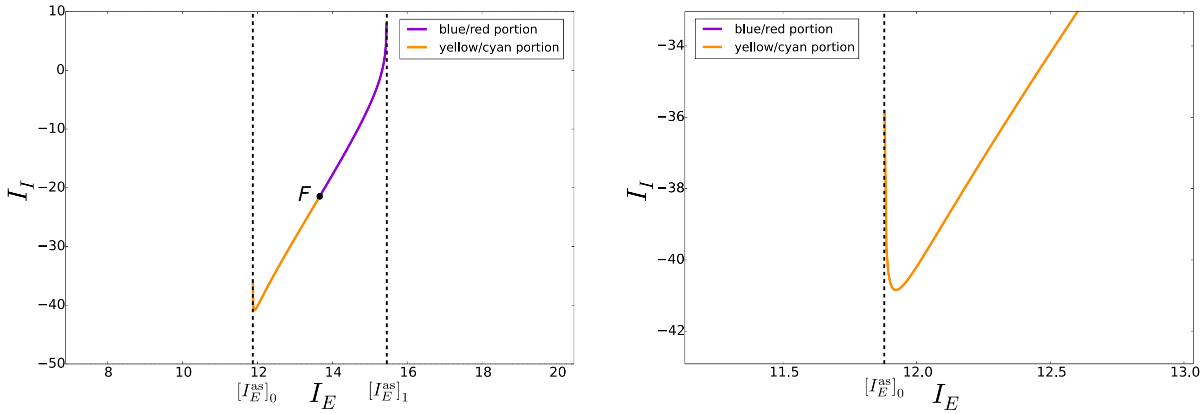


Figure S2: LP curve obtained from the perturbative expansion of the equilibrium points developed in Sec. (S2). The zoom in the right-hand side of the figure shows that the approximation does not describe the cusp bifurcation, even if the overall LP curve corresponds qualitatively to that shown in Fig. (7).

From Eq. (S7) we also observe that the orange portion of the LP curve is not defined for $-4\overline{Z}^2 - 2\overline{p} - \frac{\overline{q}}{\overline{Z}} < 0$, therefore its asymptote ($[I_E^{\mathrm{as}}]_0$, see Fig. (S2)) is obtained when $-4\overline{Z}^2 - 2\overline{p} - \frac{\overline{q}}{\overline{Z}} = 0$, and so when $\left[\mu_E^{(0)}\right]_2 = \left[\mu_E^{(0)}\right]_3 = -\frac{\overline{b}}{4\overline{a}} + \overline{Z}$, according to Eq. (S7). This last condition is satisfied when the green and yellow portions of the primary branch meet each other, and therefore when $I_E = I_E(A)$. Therefore the portion of the LP curve generated by the point $C$ converges to the portion generated by the point $A$, without ever touching it. In other terms:

$$[I_E^{\mathrm{as}}]_0 = I_E(A) \qquad \text{(S33)}$$

This is due to the fact that Eqs. (S16) + (S32) are only an approximation of the real LP curve, since they have been derived from the perturbative expansion of the equilibrium points developed in Sec. (S2). Intuitively, the divergence of $I_I$ that occurs when the orange portion approaches the point $[I_E^{\mathrm{as}}]_0$ is due to the divergence of $\mu_E^{(1)}$, contained in $\widetilde{d}$. Since $\mu_E^{(1)}$ is the only term that may explode in Eq. (S32), we conclude that it diverges also when the curve approaches the second asymptote (i.e. $[I_E^{\mathrm{as}}]_1$, see Fig. (S2)). So from Eq. (S9) we get that also $[I_E^{\mathrm{as}}]_1$ is defined by the equation $-\frac{1}{\tau_E} + \frac{N_E-1}{N-1} J_{EE} \mathscr{A}_E' \left(\mu_E^{(0)}\right) = 0$. As we know, one solution of this equation is (S15), which defines the point $A$, as it must be. The second solution is that with the $-\sqrt{\ }$ that we rejected before, namely:

$$\overline{\mu}_E^{(0)} = V_E^T - \frac{2}{\Lambda_E}\sqrt{\sqrt[3]{\left(\frac{N_E-1}{N-1} J_{EE} \frac{\nu_E^{\max}\Lambda_E}{4}\tau_E\right)^2} - 1}$$

This formula, once substituted into Eq. (S3), provides the current of the second asymptote:

$$[I_E^{\mathrm{as}}]_1 = \frac{1}{\tau_E}\overline{\mu}_E^{(0)} - \frac{N_E-1}{N-1} J_{EE} \mathscr{A}_E\left(\overline{\mu}_E^{(0)}\right) - \frac{N_I}{N-1} J_{EI}\nu_I^{\max} \qquad \text{(S34)}$$

Clearly the second LP curve of the whole codimension two bifurcation diagram (see Fig. (7)) is obtained in the same way through the approximation (S22). So we have shown that the asymptotic expansion of the equilibrium points developed in Sec. (S2) is also able to describe qualitatively the LP curve, but for a quantitative characterization of its behavior we need another approach.

For this reason now we introduce our second method for calculating analytically the LP curve. Clearly, by definition, (at least) one of the eigenvalues of the Jacobian matrix is zero at the LP points. $\lambda_E$ is always negative, and $\lambda_I < 0$ since we are in a weak-inhibition regime. Therefore we can only have $\lambda_0 = 0$ or $\lambda_1 = 0$. If $\delta + \eta < 0$, according to Eq. (S31) the condition $\lambda_0 = 0$ is equivalent to $\delta\eta = \gamma$ which, according to Eq. (S29), provides:

$$\mathscr{A}_I'\left(\mu_I\right) = \frac{-\frac{1}{\tau_E \tau_I} + \frac{1}{\tau_I}\frac{N_E-1}{N-1}J_{EE}\mathscr{A}_E'\left(\mathfrak{v}\right)}{-\frac{1}{\tau_E}\frac{N_I-1}{N-1}J_{II} + \frac{1}{(N-1)^2}\left[\left(N_E-1\right)\left(N_I-1\right)J_{EE}J_{II} - N_E N_I J_{EI}J_{IE}\right]\mathscr{A}_E'\left(\mathfrak{v}\right)} \tag{S35}$$

where we have defined the parameter $\mathfrak{v} \stackrel{\text{def}}{=} \mu_E$. Moreover, we can invert Eq. (S35) by means of Eq. (S14), obtaining:

$$\mu_I\left(\mathfrak{v}\right) = V_I^T \pm \frac{2}{\Lambda_I}\sqrt{\sqrt[3]{\left(\frac{\nu_I^{\max}\Lambda_I}{4\mathscr{A}_I'\left(\mu_I\right)}\right)^2} - 1} \tag{S36}$$

and from Eq. (5) we get:

$$\begin{cases} I_E\left(\mathfrak{v}\right) = \frac{1}{\tau_E}\mathfrak{v} - \frac{N_E-1}{N-1}J_{EE}\mathscr{A}_E\left(\mathfrak{v}\right) - \frac{N_I}{N-1}J_{EI}\mathscr{A}_I\left(\mu_I\left(\mathfrak{v}\right)\right) \\ I_I\left(\mathfrak{v}\right) = \frac{1}{\tau_I}\mu_I\left(\mathfrak{v}\right) - \frac{N_E}{N-1}J_{IE}\mathscr{A}_E\left(\mathfrak{v}\right) - \frac{N_I-1}{N-1}J_{II}\mathscr{A}_I\left(\mu_I\left(\mathfrak{v}\right)\right) \end{cases} \tag{S37}$$

So Eqs. (S35) + (S36) + (S37) define a set of parametric equations with parameter $\mathfrak{v}$ for the input currents $I_E - I_I$ that generate the LP bifurcation curve.

In the same way, if $\delta+\eta > 0$, the condition $\lambda_1 = 0$ is equivalent again to $\delta\eta = \gamma$, therefore we re-obtain the same formulas found above. These curves have been plotted in blue in Fig. (S3) (the reader may easily verify the agreement with the numerical results shown in Fig. (7)), where the part of the curve between the points $\mathrm{BT}_0$ and $\mathrm{BT}_1$, and that between the points $\mathrm{BT}_2$ and $\mathrm{BT}_3$, correspond to the case $\lambda_1 = 0$, while all the other parts are generated by the condition $\lambda_0 = 0$. At the points $\mathrm{BT}_{0,1,2,3}$, that represent the Bogdanov-Takens bifurcations, both the eigenvalues are zero, as we will see in SubSec. (S3.2.3).

Every point of the LP curve has also to satisfy the following system of inequalities:

$$\begin{cases} 0 < \mathscr{A}_I'\left(\mu_I\right) \leq \frac{\nu_I^{\max}\Lambda_I}{4} \\ \left(\delta - \eta\right)^2 + 4\gamma \geq 0 \end{cases}$$

whose solution is $\mathfrak{v} \in \left(\mathfrak{v}_a, \mathfrak{v}_b\right)$, where:

$$\mathfrak{v}_{b,a} = V_E^T \pm \frac{2}{\Lambda_E}\sqrt{\sqrt[3]{\left(\frac{N_E-1}{N-1}J_{EE}\frac{\nu_E^{\max}\Lambda_E}{4}\tau_E\right)^2} - 1} \tag{S38}$$

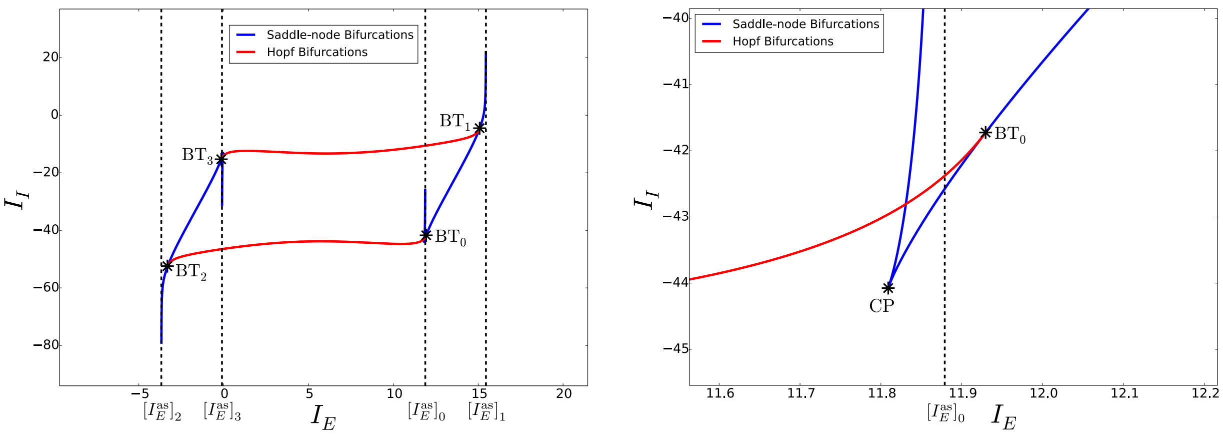


Figure S3: Analytical bifurcation diagram obtained from the eigenvalues. The zoom in the right-hand side of the figure shows the cusp bifurcation, which is not predicted by the perturbative expansion of Sec. (S2) (compare with Fig. (S2)).

Therefore we get four asymptotes $[I_E^{\mathrm{as}}]_{0,1,2,3}$ (see Fig. (S3)) for $\mathfrak{v} \to \mathfrak{v}_a^+$ and $\mathfrak{v} \to \mathfrak{v}_b^-$. In both the limiting cases we obtain $\mathscr{A}_I'(\mu_I) \to 0$ and therefore either $\mathscr{A}_I(\mu_I) \to 0$ or $\mathscr{A}_I(\mu_I) \to \nu_I^{\max}$, so the expressions of the asymptotes are:

$$\begin{aligned}
[I_E^{\mathrm{as}}]_0 &= \frac{1}{\tau_E}\mathfrak{v}_b - \frac{N_E-1}{N-1}J_{EE}\mathscr{A}_E(\mathfrak{v}_b) - \frac{N_I}{N-1}J_{EI}\nu_I^{\max} \\
[I_E^{\mathrm{as}}]_1 &= \frac{1}{\tau_E}\mathfrak{v}_a - \frac{N_E-1}{N-1}J_{EE}\mathscr{A}_E(\mathfrak{v}_a) - \frac{N_I}{N-1}J_{EI}\nu_I^{\max} \\
[I_E^{\mathrm{as}}]_2 &= \frac{1}{\tau_E}\mathfrak{v}_b - \frac{N_E-1}{N-1}J_{EE}\mathscr{A}_E(\mathfrak{v}_b) \\
[I_E^{\mathrm{as}}]_3 &= \frac{1}{\tau_E}\mathfrak{v}_a - \frac{N_E-1}{N-1}J_{EE}\mathscr{A}_E(\mathfrak{v}_a)
\end{aligned} \tag{S39}$$

We observe that $[I_E^{\mathrm{as}}]_{0,1}$ given by Eq. (S39) correspond to those provided by Eqs. (S33) and (S34), as it must be.

To conclude, we underline that even if the cusp bifurcations are evident from Fig. (S3), we cannot calculate analytically their coordinates in the codimension two bifurcation diagram. Indeed, it is possible to prove that these coordinates are given by the solutions of a high-order polynomial equation, which can be calculated only numerically.

### S3.2.2 Hopf bifurcations on the primary branch

Hopf bifurcations are defined by the existence of a simple pair of conjugate purely imaginary eigenvalues. Since $\lambda_{E,I}$ are always real, this condition can be satisfied only by $\lambda_{0,1}$, by setting $\delta + \eta = 0$ and $(\delta - \eta)^2 + 4\gamma < 0$. In particular, from the equation $\delta + \eta = 0$ we get:

$$\mathscr{A}_I'(\mu_I) = \frac{N-1}{(N_I-1)J_{II}}\left[\frac{1}{\tau_E}+\frac{1}{\tau_I}-\frac{N_E-1}{N-1}J_{EE}\mathscr{A}_E'(\mathfrak{v})\right] \tag{S40}$$

where $\mathfrak{v} \stackrel{\text{def}}{=} \mu_E$ as before. Following the same procedure introduced in SubSec. (S3.2.1), from Eq. (S40) we obtain a set of parametric equations with parameter $\mathfrak{v}$ for the input currents $I_E - I_I$ that generate the H bifurcation curve.

Every point of the curve has also to satisfy the following system of inequalities:

$$\begin{cases} 0 < \mathscr{A}_I'(\mu_I) \leq \frac{\nu_I^{\max}\Lambda_I}{4} \\ (\delta-\eta)^2 + 4\gamma < 0 \end{cases}$$

whose solution is $\mathfrak{v} \in [\mathfrak{v}_f, \mathfrak{v}_d] \cup [\mathfrak{v}_c, \mathfrak{v}_e]$, where:

$$\mathfrak{v}_{c,d} = V_E^T \pm \frac{2}{\Lambda_E}\sqrt{\sqrt[3]{\left(\frac{\nu_E^{\max}\Lambda_E(N_E-1)J_{EE}}{4(N-1)}\frac{1}{\frac{1}{\tau_E}+\frac{1}{\tau_I}-\frac{\nu_I^{\max}\Lambda_I(N_I-1)J_{II}}{4(N-1)}}\right)^2}-1}$$

$$\mathfrak{v}_{e,f} = V_E^T \pm \frac{2}{\Lambda_E}\sqrt{\sqrt[3]{\left(\frac{\nu_E^{\max}\Lambda_E}{4\mathfrak{z}}\right)^2}-1}$$

$$\mathfrak{z} = \frac{-\mathfrak{b}-\sqrt{\mathfrak{b}^2-4\mathfrak{a}\mathfrak{c}}}{2\mathfrak{a}}$$

$$\mathfrak{a} = \left(\frac{N_E-1}{N-1}J_{EE}\right)^2 - \frac{N_E N_I(N_E-1)}{(N-1)^2(N_I-1)}\frac{J_{EE}J_{EI}J_{IE}}{J_{II}}$$

$$\mathfrak{b} = -\frac{2}{\tau_E}\frac{N_E-1}{N-1}J_{EE} + \frac{N_E N_I}{(N-1)(N_I-1)}\frac{J_{EI}J_{IE}}{J_{II}}\left(\frac{1}{\tau_E}+\frac{1}{\tau_I}\right)$$

$$\mathfrak{c} = \frac{1}{\tau_E^2}$$

These curves are represented in red in Fig. (S3), and again the reader may verify the agreement with the numerical results shown in Fig. (7). It is important to observe that in Fig. (S3) we did not distinguish between subcritical and supercritical Hopf bifurcations, because the coordinates of the point GH (which, by definition, divides the two kinds of bifurcations, see [1]) cannot be calculated analytically.

### S3.2.3 Bogdanov-Takens bifurcations on the primary branch

Considering the results obtained in SubSec. (S3.2.2), the BT bifurcations are given by $\mathfrak{v} = \mathfrak{v}_{e,f}$ (equivalently, they can be obtained from the conditions $\lambda_0 = \lambda_1 = 0$, since by definition the BTs are the contact points between the LP and H curves). Therefore we get:

$$\begin{cases} I_E\left(\mathrm{BT}_0\right)=\frac{1}{\tau_E}\mathfrak{v}_e-\frac{N_E-1}{N-1}J_{EE}\mathscr{A}_E\left(\mathfrak{v}_e\right)-\frac{N_I}{N-1}J_{EI}\mathscr{A}_I\left(\mu_I^+\right) \\ I_I\left(\mathrm{BT}_0\right)=\frac{1}{\tau_I}\mu_I^+-\frac{N_E}{N-1}J_{IE}\mathscr{A}_E\left(\mathfrak{v}_e\right)-\frac{N_I-1}{N-1}J_{II}\mathscr{A}_I\left(\mu_I^+\right) \end{cases}$$

$$\begin{cases} I_E\left(\mathrm{BT}_1\right)=\frac{1}{\tau_E}\mathfrak{v}_f-\frac{N_E-1}{N-1}J_{EE}\mathscr{A}_E\left(\mathfrak{v}_f\right)-\frac{N_I}{N-1}J_{EI}\mathscr{A}_I\left(\mu_I^+\right) \\ I_I\left(\mathrm{BT}_1\right)=\frac{1}{\tau_I}\mu_I^+-\frac{N_E}{N-1}J_{IE}\mathscr{A}_E\left(\mathfrak{v}_f\right)-\frac{N_I-1}{N-1}J_{II}\mathscr{A}_I\left(\mu_I^+\right) \end{cases}$$

$$\begin{cases} I_E\left(\mathrm{BT}_2\right)=\frac{1}{\tau_E}\mathfrak{v}_e-\frac{N_E-1}{N-1}J_{EE}\mathscr{A}_E\left(\mathfrak{v}_e\right)-\frac{N_I}{N-1}J_{EI}\mathscr{A}_I\left(\mu_I^-\right) \\ I_I\left(\mathrm{BT}_2\right)=\frac{1}{\tau_I}\mu_I^--\frac{N_E}{N-1}J_{IE}\mathscr{A}_E\left(\mathfrak{v}_e\right)-\frac{N_I-1}{N-1}J_{II}\mathscr{A}_I\left(\mu_I^-\right) \end{cases}$$

$$\begin{cases} I_E\left(\mathrm{BT}_3\right)=\frac{1}{\tau_E}\mathfrak{v}_f-\frac{N_E-1}{N-1}J_{EE}\mathscr{A}_E\left(\mathfrak{v}_f\right)-\frac{N_I}{N-1}J_{EI}\mathscr{A}_I\left(\mu_I^-\right) \\ I_I\left(\mathrm{BT}_3\right)=\frac{1}{\tau_I}\mu_I^--\frac{N_E}{N-1}J_{IE}\mathscr{A}_E\left(\mathfrak{v}_f\right)-\frac{N_I-1}{N-1}J_{II}\mathscr{A}_I\left(\mu_I^-\right) \end{cases}$$

where:

$$\mu_I^{\pm}=V_I^T\pm\frac{2}{\Lambda_I}\sqrt{\sqrt[3]{\left(\frac{\nu_I^{\max}\Lambda_I\left(N_I-1\right)J_{II}}{4\left(N-1\right)\left(\frac{1}{\tau_E}+\frac{1}{\tau_I}-\frac{N_E-1}{N-1}J_{EE}\mathfrak{z}\right)}\right)^2}-1}$$

This concludes our analytical study of the local bifurcations in the weak-inhibition regime, so now we are ready to start the analysis of strong inhibition.

# S4 Strong inhibition regime

Here we study the case of strong inhibition, i.e. $\lambda_I \geq 0$. This section has a similar structure to Sec. (S3), so we start by calculating analytically the eigenvalues of the neural network (SubSec. (S4.1)), and then we will use them to derive analytically the codimension two bifurcation diagram (SubSec. (S4.2)).

## S4.1 Eigenvalues

Since in the strong-inhibition regime the inhibitory membrane potentials are in general heterogeneous (see [1]), we can reinterpret the inhibitory population as a collection of smaller inhibitory subpopulations. For this reason, in order to perform our bifurcation analysis, we need to extend the results of SubSec. (S3.1) to the case of a multi-population network. So if we consider a network with a generic number of populations $\mathfrak{P}$ and we suppose that $N_\alpha$ is the size of the population $\alpha$ (so that $\sum_{\alpha=0}^{\mathfrak{P}-1}N_\alpha=N$), the whole connectivity matrix of the system can be written as follows:

$$J=\begin{bmatrix} \mathfrak{J}_{00} & \mathfrak{J}_{01} & \cdots & \mathfrak{J}_{0,\mathfrak{P}-1} \\ \mathfrak{J}_{10} & \mathfrak{J}_{11} & \cdots & \mathfrak{J}_{1,\mathfrak{P}-1} \\ \vdots & \vdots & \ddots & \vdots \\ \mathfrak{J}_{\mathfrak{P}-1,0} & \mathfrak{J}_{\mathfrak{P}-1,1} & \cdots & \mathfrak{J}_{\mathfrak{P}-1,\mathfrak{P}-1} \end{bmatrix}, \qquad \mathfrak{J}_{\alpha\beta}=\begin{cases} J_{\alpha\alpha}\left(\mathbb{I}_{N_\alpha}-\mathrm{Id}_{N_\alpha}\right), & \text{for } \alpha=\beta \\ J_{\alpha\beta}\mathbb{I}_{N_\alpha,N_\beta}, & \text{for } \alpha\neq\beta \end{cases}$$

for $\alpha, \beta = 0, \ldots, \mathfrak{P} - 1$. The matrix $\mathfrak{J}_{\alpha\beta}$, which contains the connections from the population $\beta$ to the population $\alpha$, is $N_\alpha \times N_\beta$. So the Jacobian matrix of the system is:

$$\mathcal{J} = \begin{bmatrix} \mathscr{J}_{00} & \mathscr{J}_{01} & \cdots & \mathscr{J}_{0,\mathfrak{P}-1} \\ \mathscr{J}_{10} & \mathscr{J}_{11} & \cdots & \mathscr{J}_{1,\mathfrak{P}-1} \\ \vdots & \vdots & \ddots & \vdots \\ \mathscr{J}_{\mathfrak{P}-1,0} & \mathscr{J}_{\mathfrak{P}-1,1} & \cdots & \mathscr{J}_{\mathfrak{P}-1,\mathfrak{P}-1} \end{bmatrix}, \qquad \mathscr{J}_{\alpha\beta} = \begin{cases} -\frac{1}{\tau_\alpha}\mathrm{Id}_{N_\alpha} + \frac{J_{\alpha\alpha}}{M_\alpha}\mathscr{A}'_\alpha(\mu_\alpha)\left(\mathbb{I}_{N_\alpha} - \mathrm{Id}_{N_\alpha}\right), & \text{for } \alpha = \beta \\ \frac{J_{\alpha\beta}}{M_\alpha}\mathscr{A}'_\beta(\mu_\beta)\,\mathbb{I}_{N_\alpha,N_\beta}, & \text{for } \alpha \neq \beta \end{cases} \tag{S41}$$

where $\mu_\alpha$ are the solutions of the following system of equations:

$$-\frac{1}{\tau_\alpha}\mu_\alpha + \frac{N_\alpha - 1}{M_\alpha}J_{\alpha\alpha}\mathscr{A}_\alpha(\mu_\alpha) + \sum_{\substack{\beta=0\\ \beta\neq\alpha}}^{\mathfrak{P}-1}\frac{N_\beta}{M_\alpha}J_{\alpha\beta}\mathscr{A}_\beta(\mu_\beta) + I_\alpha = 0, \quad \alpha = 0, \ldots, \mathfrak{P}-1 \tag{S42}$$

Now we introduce the following theorem (being part of a larger work on multi-population networks, we leave it without proof, which will appear in another article).

**Theorem S1** (Eigenvalues of a multi-population network) *The Jacobian matrix S41 has eigenvalues:*

$$\lambda_\gamma = -\left[\frac{1}{\tau_\gamma} + \frac{J_{\gamma\gamma}}{M_\gamma}\mathscr{A}'_\gamma(\mu_\gamma)\right] \tag{S43}$$

*with algebraic multiplicity $N_\gamma - 1$ for $\gamma = 0, \ldots, \mathfrak{P} - 1$. The remaining $\mathfrak{P}$ eigenvalues are those of the following "reduced" $\mathfrak{P} \times \mathfrak{P}$ matrix:*

$$\mathcal{J}^R = \begin{bmatrix} \mathscr{J}^R_{00} & \mathscr{J}^R_{01} & \cdots & \mathscr{J}^R_{0,\mathfrak{P}-1} \\ \mathscr{J}^R_{10} & \mathscr{J}^R_{11} & \cdots & \mathscr{J}^R_{1,\mathfrak{P}-1} \\ \vdots & \vdots & \ddots & \vdots \\ \mathscr{J}^R_{\mathfrak{P}-1,0} & \mathscr{J}^R_{\mathfrak{P}-1,1} & \cdots & \mathscr{J}^R_{\mathfrak{P}-1,\mathfrak{P}-1} \end{bmatrix}, \qquad \mathscr{J}^R_{\alpha\beta} = \begin{cases} -\frac{1}{\tau_\alpha} + \frac{N_\alpha - 1}{M_\alpha}J_{\alpha\alpha}\mathscr{A}'_\alpha(\mu_\alpha), & \text{for } \alpha = \beta \\ \frac{N_\beta}{M_\alpha}J_{\alpha\beta}\mathscr{A}'_\beta(\mu_\beta), & \text{for } \alpha \neq \beta \end{cases} \tag{S44}$$

**Example.** The following Jacobian matrix:

$$\mathcal{J} = \begin{bmatrix} -1 & 2 & 2 & 2 & 0 & 0 & -4 & -4 & -4 \\ 2 & -1 & 2 & 2 & 0 & 0 & -4 & -4 & -4 \\ 2 & 2 & -1 & 2 & 0 & 0 & -4 & -4 & -4 \\ 2 & 2 & 2 & -1 & 0 & 0 & -4 & -4 & -4 \\ 3 & 3 & 3 & 3 & -2 & 4 & -6 & -6 & -6 \\ 3 & 3 & 3 & 3 & 4 & -2 & -6 & -6 & -6 \\ 0 & 0 & 0 & 0 & 1 & 1 & -5 & -9 & -9 \\ 0 & 0 & 0 & 0 & 1 & 1 & -9 & -5 & -9 \\ 0 & 0 & 0 & 0 & 1 & 1 & -9 & -9 & -5 \end{bmatrix}$$

represents a network with $N = 9$, $\mathfrak{P} = 3$, $N_0 = 4$, $N_1 = 2$, $N_2 = 3$, where the populations $0, 1$ are excitatory while the population 2 is inhibitory. The eigenvalues of $\mathcal{J}$ are $\lambda = -3, -6, 4$, with algebraic multiplicities $3, 1, 2$ respectively. The remaining 3 eigenvalues are those of the reduced matrix:

$$\mathcal{J}^R = \begin{bmatrix} 5 & 0 & -16 \\ 6 & 2 & -12 \\ 0 & 3 & -23 \end{bmatrix}$$

namely:

$$\lambda_0^R \approx -21.943, \qquad \lambda_{1,2}^R \approx 2.971 \pm 2.564\iota$$

As we said in [1], for the sake of clarity in this work we study the case $N_I = 2$ (for $N_I > 2$ the analysis is still feasible, but more complicated, so it is left to the interested reader). For $\lambda_I \geq 0$ the stationary solutions of the network are given by Eq. (11), which can be interpreted as a special case of Eq. (S42) in the case of three populations. So now the Jacobian matrix of the network is:

$$\mathcal{J} = \begin{bmatrix} \mathscr{J}_{00} & \mathscr{J}_{01} & \mathscr{J}_{02} \\ \mathscr{J}_{10} & \mathscr{J}_{11} & \mathscr{J}_{12} \\ \mathscr{J}_{20} & \mathscr{J}_{21} & \mathscr{J}_{22} \end{bmatrix} \tag{S45}$$

where:

$$\mathscr{J}_{00} = -\frac{1}{\tau_E}\mathrm{Id}_{N_E} + \frac{J_{EE}}{N-1}\mathscr{A}_E'(\mu_E)\left(\mathbb{I}_{N_E} - \mathrm{Id}_{N_E}\right), \quad \mathscr{J}_{01} = \frac{J_{EI}}{N-1}\mathscr{A}_I'(\mu_{I,0})\,\mathbf{1}_{N_E}, \quad \mathscr{J}_{02} = \frac{J_{EI}}{N-1}\mathscr{A}_I'(\mu_{I,1})\,\mathbf{1}_{N_E},$$

$$\mathscr{J}_{10} = \frac{J_{IE}}{N-1}\mathscr{A}_E'(\mu_E)\,\mathbf{1}_{N_E}^T, \quad \mathscr{J}_{11} = \frac{1}{\tau_I}, \quad \mathscr{J}_{12} = \frac{J_{II}}{N-1}\mathscr{A}_I'(\mu_{I,1}),$$

$$\mathscr{J}_{20} = \frac{J_{IE}}{N-1}\mathscr{A}_E'(\mu_E)\,\mathbf{1}_{N_E}^T, \quad \mathscr{J}_{21} = \frac{J_{II}}{N-1}\mathscr{A}_I'(\mu_{I,0}), \quad \mathscr{J}_{22} = \frac{1}{\tau_I}$$

Here $\mathbf{1}_{N_E}$ is the $N_E \times 1$ all-ones vector and $\mathbf{1}_{N_E}^T$ is its transpose. As we said, this allows us to reinterpret the network as if it were made of the usual excitatory population with $N_E$ neurons, and two inhibitory populations with one neuron each. According to Thm. (S1), we are in the case with $N_0 = N_E$ and $N_1 = N_2 = 1$, so the network has an eigenvalue $\lambda_E = -\left[\frac{1}{\tau_E} + \frac{J_{EE}}{N-1}\mathscr{A}_E'(\mu_E)\right]$ with multiplicity $N_E - 1$ (see Eq. (S43)), while the other eigenvalues are those of the following reduced matrix (see Eq. (S44)):

$$\mathcal{J}^R = \begin{bmatrix} -\frac{1}{\tau_E} + \frac{N_E-1}{N-1}J_{EE}\mathscr{A}_E'(\mu_E) & \frac{J_{EI}}{N-1}\mathscr{A}_I'(\mu_{I,0}) & \frac{J_{EI}}{N-1}\mathscr{A}_I'(\mu_{I,1}) \\ \frac{N_E}{N-1}J_{IE}\mathscr{A}_E'(\mu_E) & -\frac{1}{\tau_I} & \frac{J_{II}}{N-1}\mathscr{A}_I'(\mu_{I,1}) \\ \frac{N_E}{N-1}J_{IE}\mathscr{A}_E'(\mu_E) & \frac{J_{II}}{N-1}\mathscr{A}_I'(\mu_{I,0}) & -\frac{1}{\tau_I} \end{bmatrix} \tag{S46}$$

In other terms, the latter eigenvalues are the solutions of the following third-order characteristic polynomial:

$$\mathring{a}\left(\lambda^{R}\right)^{3}+\mathring{b}\left(\lambda^{R}\right)^{2}+\mathring{c}\lambda^{R}+\mathring{d}=0 \tag{S47}$$

where:

$$\begin{aligned}\mathring{a} =&1\\ \mathring{b} =&-\operatorname{tr}\left(\mathcal{J}^{R}\right)\\ \mathring{c} =&\frac{1}{2}\left\{\left[\operatorname{tr}\left(\mathcal{J}^{R}\right)\right]^{2}-\operatorname{tr}\left(\left(\mathcal{J}^{R}\right)^{2}\right)\right\}\\ \mathring{d} =&-\det\left(\mathcal{J}^{R}\right)\end{aligned} \tag{S48}$$

Now, if we define:

$$\begin{aligned}\mathring{Q} =&\sqrt[3]{\frac{\mathring{\Delta}_{1}+\sqrt{\mathring{\Delta}_{1}^{2}-4\mathring{\Delta}_{0}^{3}}}{2}}\\ \mathring{\Delta}_{0} =&\mathring{b}^{2}-3\mathring{a}\mathring{c}\\ \mathring{\Delta}_{1} =&2\mathring{b}^{3}-9\mathring{a}\mathring{b}\mathring{c}+27\mathring{a}^{2}\mathring{d}\end{aligned}$$

we get that the eigenvalues of $\mathcal{J}^{R}$ are:

$$\lambda_{k}^{R}=-\frac{1}{3\mathring{a}}\left(\mathring{b}+u_{k}\mathring{Q}+\frac{\mathring{\Delta}_{0}}{u_{k}\mathring{Q}}\right)$$

for $k=0,1,2$, where as usual $u_{0}=1$, $u_{1}=\frac{-1+\iota\sqrt{3}}{2}$, $u_{2}=\frac{-1-\iota\sqrt{3}}{2}$.

To conclude, as we already said in [1], we observe that there is an explicit relation between the inhibitory membrane potentials $\mu_{I,0}$ and $\mu_{I,1}$, that will prove very useful to determine the parametric equations of the bifurcations. So from the second and third equation of the system (11) we get:

$$-\frac{1}{\tau_{I}}\mu_{I,0}+\frac{J_{II}}{N-1}\mathscr{A}_{I}\left(\mu_{I,1}\right)=-\frac{1}{\tau_{I}}\mu_{I,1}+\frac{J_{II}}{N-1}\mathscr{A}_{I}\left(\mu_{I,0}\right)$$

This equation can be rewritten for example as follows:

$$\widehat{a}\mu_{I,1}^4+\widehat{b}\mu_{I,1}^3+\widehat{c}\mu_{I,1}^2+\widehat{d}\mu_{I,1}+\widehat{e}=0$$

where:

$$\begin{aligned}
\widehat{a}=&\frac{\Lambda_I^2}{4\tau_I^2}\\
\widehat{b}=&-\frac{\Lambda_I^2}{2\tau_I}\left(\widehat{\psi}+\frac{V_I^T}{\tau_I}\right)\\
\widehat{c}=&\frac{\Lambda_I^2}{4}\left[\widehat{\psi}^2+\left(\frac{V_I^T}{\tau_I}\right)^2+\frac{4}{\tau_I}V_I^T\widehat{\psi}\right]+\frac{1}{\tau_I^2}-\widehat{\xi}\\
\widehat{d}=&-\frac{\Lambda_I^2}{2}\widehat{\psi}V_I^T\left(\frac{V_I^T}{\tau_I}+\widehat{\psi}\right)-\frac{2}{\tau_I}\widehat{\psi}+2\widehat{\xi}V_I^T\\
\widehat{e}=&\left(\frac{\Lambda_I}{2}\widehat{\psi}V_I^T\right)^2+\widehat{\psi}^2-\widehat{\xi}\left(V_I^T\right)^2\\
\widehat{\psi}=&\frac{1}{\tau_I}\mu_{I,0}+\frac{J_{II}}{N-1}\mathscr{A}_I\left(\mu_{I,0}\right)-\frac{\nu_I^{\max}J_{II}}{2\left(N-1\right)}\\
\widehat{\xi}=&\left(\frac{\nu_I^{\max}\Lambda_I J_{II}}{4\left(N-1\right)}\right)^2
\end{aligned}$$

therefore we can express $\mu_{I,1}$ in terms of $\mu_{I,0}$ by means of the formula of the solutions of a fourth-order polynomial equation:

$$\begin{aligned}
\left[\mu_{I,1}\right]_{0,1}=&-\frac{\widehat{b}}{4\widehat{a}}-\widehat{Z}\pm\frac{1}{2}\sqrt{-4\widehat{Z}^2-2\widehat{p}+\frac{\widehat{q}}{\widehat{Z}}}\\
\left[\mu_{I,1}\right]_{2,3}=&-\frac{\widehat{b}}{4\widehat{a}}+\widehat{Z}\pm\frac{1}{2}\sqrt{-4\widehat{Z}^2-2\widehat{p}-\frac{\widehat{q}}{\widehat{Z}}}
\end{aligned} \tag{S49}$$

where the quantities $\widehat{Z}$, $\widehat{p}$, $\widehat{q}$ are defined similarly to Eq. (S8).

## S4.2 Codimension two bifurcation diagram

Now we are ready to use all the results of SubSec. (S4.1) for the evaluation of the codimension two bifurcation diagram in the strong-inhibition regime. As usual, here we cover only local bifurcations, since the global ones are analytically intractable. Of special interest is the formation of the branching points,

which are discussed in SubSec. (S4.2.1), since they represent the central topic of this article. Then in SubSec. (S4.2.2) we calculate the Zero-Hopf (neutral saddle) bifurcations, and similarly to the case of weak-inhibition, we derive analytically also the saddle-node, Hopf and Bogdanov-Takens bifurcations, respectively in SubSecs. (S4.2.3), (S4.2.4) and (S4.2.5).

### S4.2.1 Branching point bifurcations

In this subsection we study the condition $\lambda_I = 0$ that gives rise to the branching point bifurcations, namely:

$$\frac{1}{\tau_I} - \frac{|J_{II}|}{N-1} \mathscr{A}_I' \left(\mu_I \left(\mathrm{BP}\right)\right) = 0 \tag{S50}$$

The solutions of this equation are:

$$\mu_I \left(\mathrm{BP}\right) = V_I^T \pm \frac{2}{\Lambda_I} \sqrt{\sqrt[3]{\left(\frac{\tau_I \left|J_{II}\right| \nu_I^{\max} \Lambda_I}{4\left(N-1\right)}\right)^2} - 1} \tag{S51}$$

We have preferred to classify the case $\lambda_I = 0$ as an example of strong-inhibition regime, since it describes the formation of the secondary branches on which new bifurcations will arise for $\lambda_I > 0$, as we will discuss in the next part of the article. Being a limiting case, the condition $\lambda_I = 0$ can be studied either from Eq. (5) or equivalently from Eq. (11) after setting $\mu_{I,0} = \mu_{I,1}$. So for example, if we choose to use Eq. (5), from its second equation we get:

$$\mu_E \left(\mathrm{BP}\right) = V_E^T \pm \frac{2}{\Lambda_E} \sqrt{\frac{1}{\frac{1}{\left\{\frac{2(N-1)}{\nu_E^{\max} N_E J_{IE}} \left[\frac{1}{\tau_I} \mu_I(\mathrm{BP}) - \frac{N_I - 1}{N-1} J_{II} \mathscr{A}_I(\mu_I(\mathrm{BP})) - I_I\right] - 1\right\}^2} - 1}} \tag{S52}$$

while from its first equation we obtain:

$$I_E = \frac{1}{\tau_E} \mu_E \left(\mathrm{BP}\right) - \frac{N_E - 1}{N-1} J_{EE} \mathscr{A}_E \left(\mu_E \left(\mathrm{BP}\right)\right) - \frac{N_I}{N-1} J_{EI} \mathscr{A}_I \left(\mu_I \left(\mathrm{BP}\right)\right) \tag{S53}$$

where $\mu_E\left(\mathrm{BP}\right)$ and $\mu_I\left(\mathrm{BP}\right)$ are given by Eqs. (S51) and (S52) respectively. Since $\mu_E\left(\mathrm{BP}\right)$ depends on $I_I$, Eq. (S53) defines explicit functions $I_E = \mathcal{F}\left(I_I\right)$ that provide all the pairs $I_E - I_I$ at which a branching point bifurcation occurs. Now from Eq. (S51) we observe that $\mu_I\left(\mathrm{BP}\right)$ has two different possible values depending on the sign in front of the square root, while from Eq. (S52) we see that $\mu_E\left(\mathrm{BP}\right)$ has four possible solutions, due to the sign of the square root and to the value of $\mu_I\left(\mathrm{BP}\right)$. However, only the pairs $\left(\mu_E\left(\mathrm{BP}\right) = V_E^T + \ldots, \mu_I^-\left(\mathrm{BP}\right) \stackrel{\mathrm{def}}{=} V_I^T - \ldots\right)$ and $\left(\mu_E\left(\mathrm{BP}\right) = V_E^T - \ldots, \mu_I^+\left(\mathrm{BP}\right) \stackrel{\mathrm{def}}{=} V_I^T + \ldots\right)$, where $\mu_E\left(\mathrm{BP}\right)$ is calculated from the $\mu_I\left(\mathrm{BP}\right)$ of the corresponding pair through Eq. (S52), satisfy the system (5). These pairs of membrane potentials, once replaced into Eq. (S53), define two functions that we call $I_E = \mathcal{F}_-\left(I_I\right)$ and $I_E = \mathcal{F}_+\left(I_I\right)$ respectively. Moreover, from Eqs. (S51) and (S52) we see that these functions exist if and only if:

$$\begin{cases} \frac{\tau_I |J_{II}| \nu_I^{\max} \Lambda_I}{4(N-1)} \geq 1 \\ \frac{1}{\frac{1}{\left\{\frac{2(N-1)}{\nu_E^{\max} N_E J_{IE}} \left[\frac{1}{\tau_I} \mu_I (\mathrm{BP}) - \frac{N_I - 1}{N-1} J_{II} \mathscr{A}_I (\mu_I (\mathrm{BP})) - I_I\right] - 1\right\}^2} - 1} \geq 0 \\ \left\{\frac{2(N-1)}{\nu_E^{\max} N_E J_{IE}} \left[\frac{1}{\tau_I} \mu_I (\mathrm{BP}) - \frac{N_I - 1}{N-1} J_{II} \mathscr{A}_I (\mu_I (\mathrm{BP})) - I_I\right] - 1\right\}^2 \neq 1 \end{cases}$$

from which we obtain that $\mathcal{F}_-$ is defined for $[I_I^{\text{as}}]_0 < I_I < [I_I^{\text{as}}]_1$, while $\mathcal{F}_+$ for $[I_I^{\text{as}}]_2 < I_I < [I_I^{\text{as}}]_3$, where:

$$\begin{aligned} [I_I^{\text{as}}]_0 =& \frac{1}{\tau_I} \mu_I^- (\mathrm{BP}) - \frac{N_I - 1}{N-1} J_{II} \mathscr{A}_I \left(\mu_I^- (\mathrm{BP})\right) - \frac{\nu_E^{\max} N_E J_{IE}}{N-1} \\ [I_I^{\text{as}}]_1 =& \frac{1}{\tau_I} \mu_I^- (\mathrm{BP}) - \frac{N_I - 1}{N-1} J_{II} \mathscr{A}_I \left(\mu_I^- (\mathrm{BP})\right) \\ [I_I^{\text{as}}]_2 =& \frac{1}{\tau_I} \mu_I^+ (\mathrm{BP}) - \frac{N_I - 1}{N-1} J_{II} \mathscr{A}_I \left(\mu_I^+ (\mathrm{BP})\right) - \frac{\nu_E^{\max} N_E J_{IE}}{N-1} \\ [I_I^{\text{as}}]_3 =& \frac{1}{\tau_I} \mu_I^+ (\mathrm{BP}) - \frac{N_I - 1}{N-1} J_{II} \mathscr{A}_I \left(\mu_I^+ (\mathrm{BP})\right) \end{aligned}$$

So the horizontal asymptotes $[I_I^{\text{as}}]_{0,1,2,3}$ define the domain of the two functions $\mathcal{F}_\pm$ and describe the behavior of the branching point curves for large values of $|I_E|$ (compare with Fig. (10)).

### S4.2.2 Zero-Hopf (neutral saddle) bifurcations

By definition, the ZH bifurcations are obtained when the network has a zero eigenvalue and a pair of conjugate purely imaginary eigenvalues. In our case, this occurs at the intersection of the BP and H curves, therefore the ZH bifurcations satisfy the following conditions (see Eqs. (S40) and (S50)):

$$\begin{cases} \mathscr{A}_I' (\mu_I (\mathrm{ZH})) = \frac{N-1}{(N_I - 1) J_{II}} \left[\frac{1}{\tau_E} + \frac{1}{\tau_I} - \frac{N_E - 1}{N-1} J_{EE} \mathscr{A}_E' (\mu_E (\mathrm{ZH}))\right] \\ \frac{1}{\tau_I} - \frac{|J_{II}|}{N-1} \mathscr{A}_I' (\mu_I (\mathrm{ZH})) = 0 \end{cases}$$

From this system of equations we get:

$$\begin{aligned} \mathscr{A}_E' (\mu_E (\mathrm{ZH})) =& \frac{N-1}{(N_E - 1) J_{EE}} \left(\frac{1}{\tau_E} + \frac{N_I}{\tau_I}\right) \\ \mathscr{A}_I' (\mu_I (\mathrm{ZH})) =& \frac{N-1}{\tau_I |J_{II}|} \end{aligned}$$

and therefore:

$$\mu_E^{\pm}(\mathrm{ZH}) = V_E^T \pm \frac{2}{\Lambda_E}\sqrt{\sqrt[3]{\left(\frac{\nu_E^{\max}\Lambda_E(N_E-1)J_{EE}}{4(N-1)\left(\frac{1}{\tau_E}+\frac{N_I}{\tau_I}\right)}\right)^2}-1}$$

$$\mu_I^{\pm}(\mathrm{ZH}) = V_I^T \pm \frac{2}{\Lambda_I}\sqrt{\sqrt[3]{\left(\frac{\nu_I^{\max}\Lambda_I\tau_I|J_{II}|}{4(N-1)}\right)^2}-1} \tag{S54}$$

So finally, from Eq. (5) or (11), we see that the coordinates of the ZH bifurcations are:

$$\begin{cases} I_E(\mathrm{ZH}_0) = \frac{1}{\tau_E}\mu_E^+(\mathrm{ZH}) - \frac{N_E-1}{N-1}J_{EE}\mathscr{A}_E\left(\mu_E^+(\mathrm{ZH})\right) - \frac{N_I}{N-1}J_{EI}\mathscr{A}_I\left(\mu_I^+(\mathrm{ZH})\right) \\ I_I(\mathrm{ZH}_0) = \frac{1}{\tau_I}\mu_I^+(\mathrm{ZH}) - \frac{N_E}{N-1}J_{IE}\mathscr{A}_E\left(\mu_E^+(\mathrm{ZH})\right) - \frac{N_I-1}{N-1}J_{II}\mathscr{A}_I\left(\mu_I^+(\mathrm{ZH})\right) \end{cases}$$

$$\begin{cases} I_E(\mathrm{ZH}_1) = \frac{1}{\tau_E}\mu_E^-(\mathrm{ZH}) - \frac{N_E-1}{N-1}J_{EE}\mathscr{A}_E\left(\mu_E^-(\mathrm{ZH})\right) - \frac{N_I}{N-1}J_{EI}\mathscr{A}_I\left(\mu_I^+(\mathrm{ZH})\right) \\ I_I(\mathrm{ZH}_1) = \frac{1}{\tau_I}\mu_I^+(\mathrm{ZH}) - \frac{N_E}{M_I}J_{IE}\mathscr{A}_E\left(\mu_E^-(\mathrm{ZH})\right) - \frac{N_I-1}{N-1}J_{II}\mathscr{A}_I\left(\mu_I^+(\mathrm{ZH})\right) \end{cases}$$

$$\begin{cases} I_E(\mathrm{ZH}_2) = \frac{1}{\tau_E}\mu_E^+(\mathrm{ZH}) - \frac{N_E-1}{N-1}J_{EE}\mathscr{A}_E\left(\mu_E^+(\mathrm{ZH})\right) - \frac{N_I}{N-1}J_{EI}\mathscr{A}_I\left(\mu_I^-(\mathrm{ZH})\right) \\ I_I(\mathrm{ZH}_2) = \frac{1}{\tau_I}\mu_I^-(\mathrm{ZH}) - \frac{N_E}{N-1}J_{IE}\mathscr{A}_E\left(\mu_E^+(\mathrm{ZH})\right) - \frac{N_I-1}{N-1}J_{II}\mathscr{A}_I\left(\mu_I^-(\mathrm{ZH})\right) \end{cases}$$

$$\begin{cases} I_E(\mathrm{ZH}_3) = \frac{1}{\tau_E}\mu_E^-(\mathrm{ZH}) - \frac{N_E-1}{N-1}J_{EE}\mathscr{A}_E\left(\mu_E^-(\mathrm{ZH})\right) - \frac{N_I}{N-1}J_{EI}\mathscr{A}_I\left(\mu_I^-(\mathrm{ZH})\right) \\ I_I(\mathrm{ZH}_3) = \frac{1}{\tau_I}\mu_I^-(\mathrm{ZH}) - \frac{N_E}{N-1}J_{IE}\mathscr{A}_E\left(\mu_E^-(\mathrm{ZH})\right) - \frac{N_I-1}{N-1}J_{II}\mathscr{A}_I\left(\mu_I^-(\mathrm{ZH})\right) \end{cases}$$

In the current and in the previous subsection we have studied the case $\lambda_I = 0$. From now on we will restrict ourselves to the case $\lambda_I > 0$.

### S4.2.3 Saddle-node bifurcations on the secondary branches

The LP curve that occurs on the secondary branches is given by the condition that (at least) one eigenvalue of the Jacobian matrix (S45) is equal to zero. Since the determinant of a matrix is equal to the product of its eigenvalues, and moreover the eigenvalues $\lambda_E$ are never equal to zero, then the LP curve is described by the equation $\det\left(\mathcal{J}^R\right) = 0$. After some algebra, this condition can be rewritten as $\acute{a}\mathscr{A}_E'(\mu_E) - \acute{b} = 0$, where:

$$\begin{aligned} \acute{a} =& \frac{1}{\tau_I^2}\frac{N_E-1}{N-1}J_{EE} + \frac{1}{\tau_I}\frac{N_E}{(N-1)^2}J_{EI}J_{IE}\left[\mathscr{A}_I'(\mu_{I,0}) + \mathscr{A}_I'(\mu_{I,1})\right] \\ &+ \frac{1}{(N-1)^3}\left[2N_EJ_{EI}J_{IE}J_{II} - (N_E-1)J_{EE}J_{II}^2\right]\mathscr{A}_I'(\mu_{I,0})\mathscr{A}_I'(\mu_{I,1}) \\ \acute{b} =& \frac{1}{\tau_E}\left[\frac{1}{\tau_I^2} - \left(\frac{J_{II}}{N-1}\right)^2\mathscr{A}_I'(\mu_{I,0})\mathscr{A}_I'(\mu_{I,1})\right] \end{aligned} \tag{S55}$$

| $J_{II}$ | $\mathfrak{v}_{\min}$ | $\mathfrak{v}_{\max}$ |
|---|---|---|
| −80 | 5.76 | 6.89 |
| −100 | 5.42 | 9.42 |
| −200 | 5.33 | 20.41 |
| −300 | 5.32 | 31.30 |
| −400 | 5.32 | 42.18 |

Table S1: Range of the parameter $\mathfrak{v} \stackrel{\mathrm{def}}{=} \mu_{I,0}$ obtained numerically from Eq. (S57), for different values of $J_{II}$. We observe that for large $|J_{II}|$ the parameter $\mathfrak{v}_{\min}$ reaches a constant value, while $\mathfrak{v}_{\max}$ increases linearly. This result suggests that simple asymptotic expressions of $\mathfrak{v}_{\min}$ and $\mathfrak{v}_{\max}$ can be derived analytically. Nevertheless this calculation is beyond the purpose of the article, and is left to the interested reader.

so we get:

$$\mathscr{A}_E'(\mu_E) = \frac{\acute{b}}{\acute{a}} \tag{S56}$$

Now, by inverting Eq. (S56), we obtain $\mu_E$ as a function of $\acute{a}$, $\acute{b}$, that in turn depend on $\mu_{I,0}$ and $\mu_{I,1}$. Combining this result with Eq. (S49), we get $\mu_E$ as a function of $\mu_{I,0}$ only, which can be used to get the parametric equations of the LP curve. Indeed, if we define $\mathfrak{v} \stackrel{\mathrm{def}}{=} \mu_{I,0}$, now we have formulas $\mu_E^{\pm} = f_{\pm}(\mathfrak{v})$ (depending on the sign in the expression $\mu_E^{\pm} = V_E^T \pm \cdots$) and $\mu_{I,1} = g(\mathfrak{v})$, which replaced in Eq. (11) provide the parametric equations of the currents $I_{E,I}$ on the LP curve, as a function of the parameter $\mathfrak{v}$.

In particular, it turns out that the two portions of the LP curve are generated by $[\mu_{I,1}]_1$ (see Eq. (S49)), therefore the points on these curves have to satisfy the following system of inequalities:

$$\begin{cases} 0 < \mathscr{A}_E'(\mu_E) \leq \frac{\nu_E^{\max}\Lambda_E}{4} \\ 0 < \mathscr{A}_I'(\mu_I) \leq \frac{\nu_I^{\max}\Lambda_I}{4} \\ -4\widehat{Z}^2 - 2\widehat{p} + \frac{\widehat{q}}{\widehat{Z}} \geq 0 \end{cases} \tag{S57}$$

The system (S57) determines the range of $\mathfrak{v}$ where the LP curve is defined, but unfortunately it cannot be solved explicitly. However, in this case the extremes of the range of $\mathfrak{v}$ do not define any important codimension two bifurcation point or asymptote, differently to what occurs for the LP curve on the primary branch. For this reason their exact evaluation is not fundamental. Nevertheless, for the sake of completeness some numerical examples are shown in Tab. (S1) for different values of $J_{II}$.

From the formula of $\acute{b}$ it is interesting to observe that $\mathscr{A}_E'(\mu_E)$ is proportional to $\frac{1}{\tau_I^2} - \left(\frac{J_{II}}{N-1}\right)^2 \mathscr{A}_I'(\mu_{I,0})\mathscr{A}_I'(\mu_{I,1})$. Since for $\lambda_I \to 0$ we get $\mu_{I,0} \to \mu_{I,1}$, and since $\frac{1}{\tau_I^2} - \left(\frac{J_{II}}{N-1}\mathscr{A}_I'(\mu_{I,0})\right)^2 = -\lambda_I\left(\frac{1}{\tau_I} - \frac{J_{II}}{N-1}\mathscr{A}_I'(\mu_{I,0})\right)$, we conclude that $\lambda_I = 0$ implies $\mathscr{A}_E'(\mu_E) = 0$. In other terms, according to our analytical formula the LP curve on the secondary branches cannot exist for $\lambda_I = 0$, as it must be.

To conclude, we observe that on the LP curve we have new CP bifurcations, whose coordinates cannot be calculated analytically, as in the case of the primary branch.

### S4.2.4 Hopf bifurcations on the secondary branches

If we replace $\lambda^R = \pm \iota\omega$ into Eq. (S47), we get the following system of equations:

$$\begin{cases} \mathring{a}\omega^3 - \mathring{c}\omega = 0 \\ \mathring{b}\omega^2 - \mathring{d} = 0 \end{cases}$$

$\omega = 0$ is a solution if and only if $\mathring{d} = 0$ (this corresponds to the BT bifurcation that will be discussed later in SubSec. (S4.2.5)). Moreover, the remaining solution $\omega \neq 0$ exists if and only if $\mathring{a}\mathring{d} - \mathring{b}\mathring{c} = 0$. By means of Eq. (S48), after some algebra this last condition can be written more explicitly as $\grave{a}\left(\mathscr{A}_E'\left(\mu_E\right)\right)^2 + \grave{b}\mathscr{A}_E'\left(\mu_E\right) + \grave{c} = 0$, where:

$$\begin{aligned}
\grave{a} =& \frac{N_E - 1}{N-1} J_{EE} \left[\frac{2}{\tau_I}\frac{N_E-1}{N-1}J_{EE} + \frac{N_E}{(N-1)^2} J_{EI} J_{IE} \left(\mathscr{A}_I'\left(\mu_{I,0}\right) + \mathscr{A}_I'\left(\mu_{I,1}\right)\right)\right] \\
\grave{b} =& 2\frac{N_E}{(N-1)^3} J_{EI} J_{IE} J_{II} \mathscr{A}_I'\left(\mu_{I,0}\right)\mathscr{A}_I'\left(\mu_{I,1}\right) - \left(\frac{1}{\tau_E} + \frac{1}{\tau_I}\right)\left[\frac{4}{\tau_I}\frac{N_E-1}{N-1}J_{EE} + \frac{N_E}{(N-1)^2} J_{EI} J_{IE}\left(\mathscr{A}_I'\left(\mu_{I,0}\right) + \mathscr{A}_I'\left(\mu_{I,1}\right)\right)\right] \\
\grave{c} =& \frac{2}{\tau_I}\left[\left(\frac{1}{\tau_E} + \frac{1}{\tau_I}\right)^2 - \left(\frac{J_{II}}{N-1}\right)^2 \mathscr{A}_I'\left(\mu_{I,0}\right)\mathscr{A}_I'\left(\mu_{I,1}\right)\right]
\end{aligned} \tag{S58}$$

So we get:

$$\mathscr{A}_E'\left(\mu_E^{\pm}\right) = \frac{-\grave{b} \pm \sqrt{\grave{b}^2 - 4\grave{a}\grave{c}}}{2\grave{a}} \tag{S59}$$

From now on, we can follow the same procedure explained in SubSec. (S4.2.3) for the LP curve, ending up with a parametric formula for the H curves on the secondary branches.

As usual, we need to find also the range of the parameter $\mathfrak{v} = \mu_{I,0}$. As for the LP curve that we discussed before, this range cannot be calculated analytically. However, in some cases one of the extremes of the range can be found. Indeed, in Fig. (10) we showed that when inhibition is strong enough, the H curves of the secondary branches are connected to the BP curves through the same ZH bifurcation points that we calculated in SubSec. (S4.2.2), and whose inhibitory membrane potentials are known (see Eq. (S54)). Now we want to prove briefly that the H curves of the secondary branches actually converge to the ZH points, when they exist. For $\lambda_I \to 0$ we know that $\mu_{I,0}$ and $\mu_{I,1}$ converge to the inhibitory potential $\mu_I$ of the primary branch, therefore the reduced Jacobian matrix (S46) becomes:

$$\mathcal{J}^R = \begin{bmatrix} -\frac{1}{\tau_E} + \frac{N_E-1}{N-1} J_{EE}\mathscr{A}_E'\left(\mu_E\right) & \frac{J_{EI}}{N-1}\mathscr{A}_I'\left(\mu_I\right) & \frac{J_{EI}}{N-1}\mathscr{A}_I'\left(\mu_I\right) \\ \frac{N_E}{N-1} J_{IE}\mathscr{A}_E'\left(\mu_E\right) & -\frac{1}{\tau_I} & -\frac{1}{\tau_I} \\ \frac{N_E}{N-1} J_{IE}\mathscr{A}_E'\left(\mu_E\right) & -\frac{1}{\tau_I} & -\frac{1}{\tau_I} \end{bmatrix}$$

It is easy to prove that this matrix has eigenvalues $\lambda_0^R = \lambda_I = 0$ and $\lambda_{1,2}^R = \lambda_{0,1}$, where $\lambda_{0,1}$ are given by Eq. (S31). In other words, for $\lambda_I \to 0$ the two conjugate purely imaginary eigenvalues $\lambda_{1,2}^R$ converge to $\lambda_{0,1}$. This means that the H curves of the secondary branch meet the BP curve when two eigenvalues

are conjugate purely imaginary and equal to those of the primary branch. As we know, the latter is the condition that defines the H curves of the primary branch. Therefore the H curves of the primary and secondary branches and the BP curve meet each other at the same point, which must be ZH, according to the results in SubSec. (S4.2.2). So one of the extremes of the parameter for each H curve is $\mathfrak{v} = \mu_I$ (ZH), as given by Eq. (S54), while the other must be calculated numerically.

We conclude by observing that the point GH is analytically intractable, as in the case of weak inhibition.

#### S4.2.5 Bogdanov-Takens bifurcations on the secondary branches

The BT bifurcations occur at the intersection between the LP and H curves, therefore they are defined by Eqs. (S56) and (S59) taken into account together. From them we obtain the condition:

$$\grave{a}\acute{b}^2 + \acute{a}\grave{b}\acute{b} + \acute{a}^2\grave{c} = 0 \tag{S60}$$

Now, these parameters are functions of $\mu_{I,0}$ and $\mu_{I,1}$ (see Eqs. (S55) and (S58)), therefore from Eqs. (S49) and (S60) we obtain two equations in two unknowns, from which in principle we should be able to obtain the inhibitory membrane potentials. However, these equations turn out to be analytically intractable. For this reason, the BT bifurcations can be calculated only numerically. The simplest way is by checking when the condition $\mathring{d} = 0$ is satisfied on the H curves of the secondary branches, because this corresponds to find the points where the H and LP curves meet each other. Alternatively, it also possible to check the condition $\mathring{c} = 0$, since $\mathring{a}\mathring{d} - \mathring{b}\mathring{c} = 0$ on the H curves and $\mathring{b} \neq 0$ (with the exception of the ZH points, where $\mathring{b} = -\mathrm{tr}\left(\mathcal{J}^R\right) = -\left(0 + \lambda_0 + \lambda_1\right) = 0$).

# S5 Examples of dynamics from the codimension two bifurcation diagram

The codimension two bifurcation diagrams shown in Figs. (7) and (10) contain almost all the information concerning the dynamics the model is able to exhibit for different values of $J_{II}$. However, the knowledge about the amplitudes of the oscillations, as well as the value of the membrane potentials at the equilibrium points and their stability, is carried out by the codimension one diagrams. For this reason, by following the same logical path as in [3], in this section we integrate the results shown in [1] by providing the codimension one bifurcation diagrams for several values of $I_I$ in both the weak and strong-inhibition regimes (see SubSecs. (S5.1) and (S5.2) respectively).

## S5.1 Weak-inhibition regime

Let us first consider the weak-inhibition regime, in the case $J_{II} = -10$. Due to the high symmetry in the bifurcation diagram of the system (see Fig. (7)), we focus on its upper-half part, as shown in Fig. (S4).

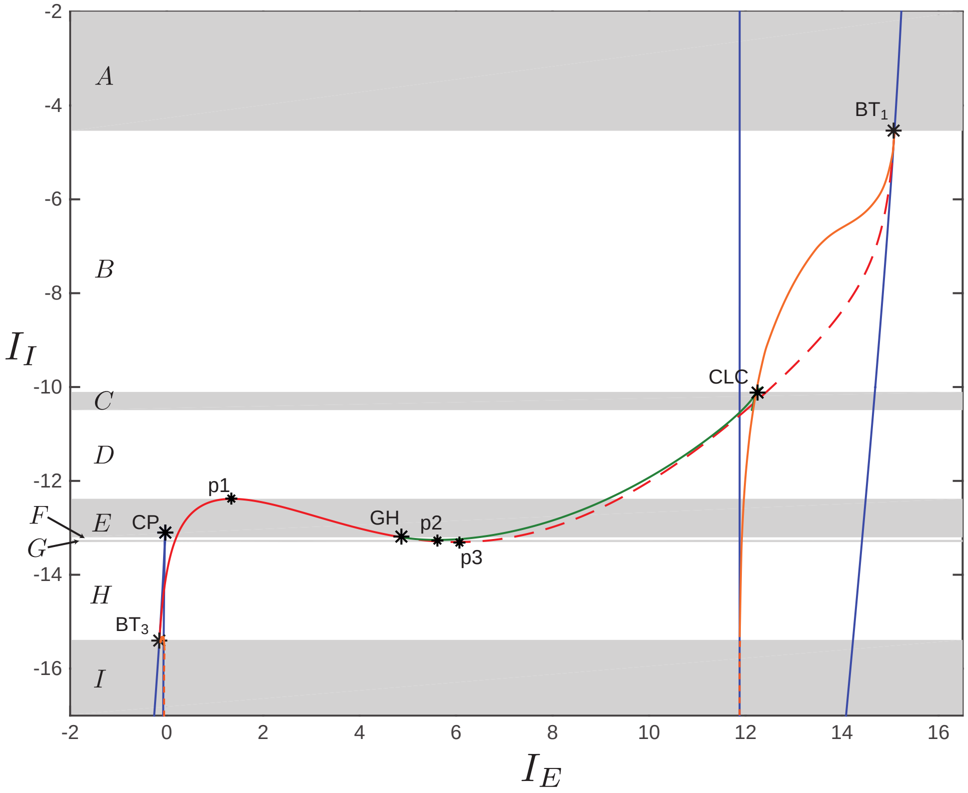


Figure S4: Due to the high symmetry of the codimension two bifurcation diagram shown in Fig. (7), we focus here on its upper-half part. In addition to the codimension two bifurcations presented in Fig. (7), we consider three additional points p1, p2, p3 that allow us to divide the diagram horizontally in nine areas, identified by the letters A-I. The codimension one bifurcation diagram of each slice is shown in Fig. (S5). For the meaning of the colors see [1].

The codimension two bifurcation points, with the addition of the relative maxima and minima of the H and limit point of cycles curves (identified by the labels p1, p2 and p3), provide a subdivision of the $I_E - I_I$ plane, which is also detectable by white and gray backgrounds. Specifically, we find nine areas, identified by the letters A-I, where the system exhibits qualitatively similar dynamics. Overall, the system displays temporal behavior which is of considerable physiological interest. In particular, we stress the presence of damped oscillations, stable oscillations and hysteresis. Damped oscillations are involved in the thalamus, in the olfactory bulb and in the cortex [4–7] as a reaction to impulse stimulation. Moreover, stable oscillatory activity is an emerging property of the thalamocortical system and can be observed at the macroscopic scale in EEG signals [8]. It is commonly classified in the frequency bands delta (1-4 Hz), theta (4-8 Hz), alpha (8-13 Hz), beta (13-30 Hz) and gamma (30-80 Hz). Slow and infra-slow oscillations (0.1-1 Hz and 0.02-0.1 Hz respectively) can also be observed, as well as fast and ultra-fast rhythms (80-200 Hz and 200-600 Hz) [9].

It is important to observe that our model, as described by Eq. (3), is dimensionless. In order to match it with neurophysiological recordings, it is natural to express the membrane potentials in mV. Moreover, since in our analysis we chose $\tau_E = \tau_I = 1$ (see Tab. (1)), and since the membrane time constant of biological neurons is of the order of 10 ms (see for example [10]), we conclude that in our simulations time is expressed in centiseconds. For this reason, if numerical simulations exhibits oscillations with dimensionless frequency $f_{\mathrm{num}}$, the corresponding frequency in physical units is $100 \times f_{\mathrm{num}}$ Hz.

By going into the details of our analysis, below we list all the areas highlighted in Fig. (S4), and we describe their corresponding codimension one bifurcation diagrams. The collection of these diagrams is shown in Fig. (S5), where each panel describes the equilibrium points in the excitatory population as a function of $I_E$, while $I_I$ is held constant (the equilibria of the inhibitory population have been omitted due to the similarity with those of the excitatory population).

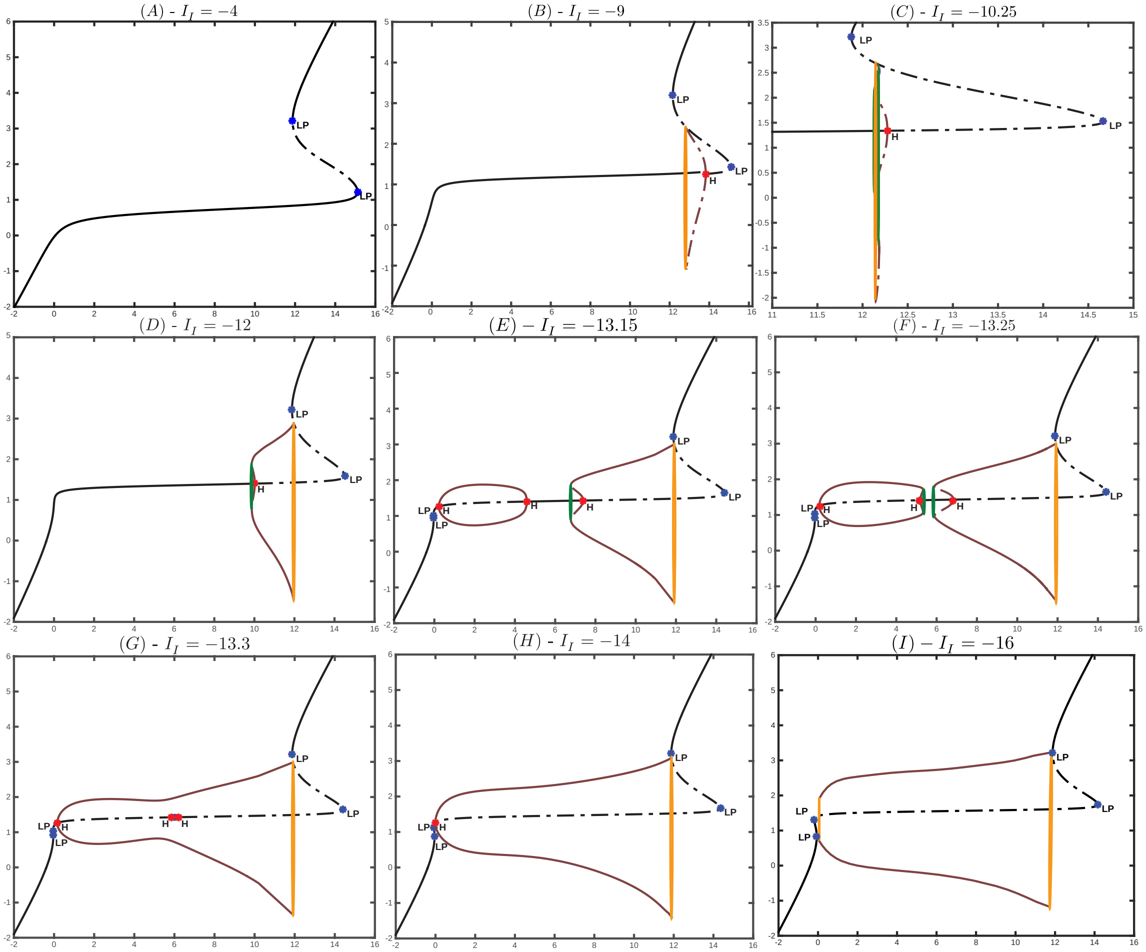


Figure S5: Each panel of this figure describes $\mu_E$ on the vertical axis as a function of $I_E$ on the horizontal axis (the panels of $\mu_I$ have been omitted, see text), for different values of $I_I$ in areas A-I. The stable/unstable equilibrium curves are described by plain/dashed black lines. Limit point (LP), as well as Andronov-Hopf (H) bifurcations, lie on the equilibrium curve. Supercritical/subcritical Andronov-Hopf bifurcations give rise to stable/unstable limit cycles described by plain/dashed brown curves. Homoclines, that are characterized by large amplitude limit cycles with infinite period, are described by orange loops. The green loops identify the values of the current at which the limit cycles cross the Limit Point of Cycles bifurcations. Here, limit cycles change stability.

In Fig. (S4), we identify the bounds of each area on the $I_I$-axis by the notation $I_I(\mathcal{B})$, where $\mathcal{B}$ represents the bifurcation acronym; moreover, $I_I(\mathrm{LB}) = -17$ and $I_I(\mathrm{UB}) = -2$ characterize the lower and upper bounds, respectively, of the inhibitory current of the whole diagram.

**[A-B]** For $I_I(\mathrm{CLC}) < I_I < I_I(\mathrm{UB})$, areas A and B are characterized by non-oscillating activity (motivated by the absence of stable limit cycles) and bistability. Nonetheless, stable equilibrium points,

both foci and nodes, exist. The unstable equilibrium points and the unstable limit cycles create basin separatrixes that determine, depending on the initial conditions, the equilibrium to which the solutions converge. In particular, the lower stable portion of the equilibrium curve is characterized by a low firing rate activity, and since the eigenvalues are complex-conjugate, these equilibria are foci. This means that for all the initial conditions belonging to the basin of attraction of the low-activity state, damped oscillations appear. On the contrary, the higher stable portion of the equilibrium curve corresponding to the high firing activity is characterized by real eigenvalues and thus is constituted by nodes. Examples of time evolution of the membrane potentials that converge to foci, as well as to stable nodes, are represented in Fig. (S6), left.

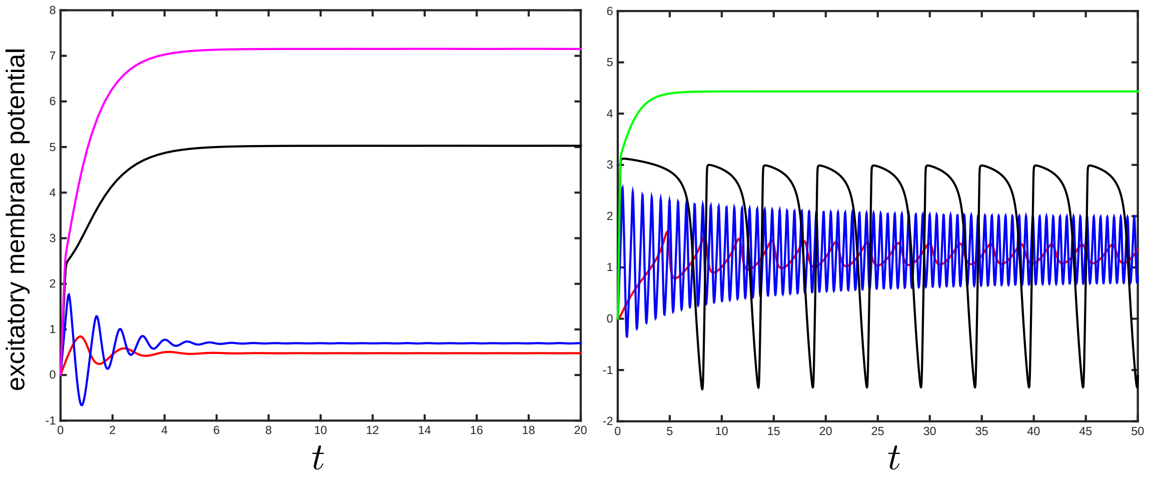


Figure S6: Time evolution of the excitatory membrane potentials $V_i(t)$ (for any $i = 0, \ldots, N_E - 1$), obtained from Eq. (3) for different values of the external currents. Left, we fix $I_I = -4$ (area A in Fig. (S5)). For $I_E = 2$ and $I_E = 7$ the solutions converge to stable foci, giving rise to damped oscillations (red and blue curve, respectively). For $I_E = 13$ and $I_E = 15$ the solutions converge to stable nodes (black and purple curve, respectively). Right, we fix $I_I = -13.3$ (area G in Fig. (S5)). For $I_E = 0.216$ we find low-amplitude oscillations of about 35 Hz (red curve). For $I_E = 5.564$ the amplitude of the oscillations is larger than the previous case, and the frequency increases up to 160 Hz (blue curve). High-amplitude oscillations occur for $I_E = 11.85$; since this current is close to that of the homoclinic bifurcation, the frequency decays to 19 Hz (black curve). Finally, for $I_E = 12.5$ the system reaches a stable node (green curve).

Furthermore, bistability is present in both the bifurcation diagrams in areas A-B. As we said in SubSec. (3.2), in A bistability occurs in presence of hysteresis.

**[C-I]** Stable oscillations with different frequencies are present for all $I_I(\mathrm{BT}_3) < I_I < I_I(\mathrm{CLC})$. However, they are generated by different kinds of bifurcations. In more details, in area C the subcritical Andronov-Hopf bifurcation gives rise to unstable limit cycles. Due to the vicinity to the cusp of limit point of cycles (CLC), the limit point of cycle curve is two-fold crossed and leads the unstable limit cycles to become stable and hereafter unstable again. Finally, they vanish in a homoclinic bifurcation where the frequency of the oscillations decays to 0 Hz. Thus, in a narrow range of values of $I_E$, three stable solutions coexist: a damped oscillating solution and a non-oscillating solution, as in the areas A-B, together with stable oscillations in the range of about 30-128 Hz. Furthermore, in area D, stable limit cycles originate from the unstable ones after reaching the limit point of cycles curve. These stable limit cycles reach the maximum oscillation frequency just after they change stability; its value is about 150 Hz. The stable limit cycles vanish in the homoclinic bifurcation. Finally, in the remaining areas E-H, we always observe oscillatory activity described by one or two families of stable limit cycles. In all the

cases, the frequencies span from the theoretical 0 Hz at the homoclinic bifurcation up to 170 Hz. Several examples of oscillations are shown in Fig. (S6), right.

To conclude, for $I_I\,(\mathrm{LB}) < I_I < I_I\,(\mathrm{BT}_3)$ the system presents both stable equilibrium points and stable limit cycles. In particular, stable equilibria describe states with high firing-rates for large $I_E$. On the contrary, states with low firing-rates emerge for low $I_E$. Moreover, for intermediate values of $I_E$, the unstable equilibria are surrounded by stable limit cycles. In turn, the stable limit cycles are enclosed between two homoclinic bifurcations.

## S5.2 Strong-inhibition regime

Let us now consider the strong-inhibition regimes $J_{II} = -34$ and $J_{II} = -100$. The codimension two bifurcation diagrams in these cases are more complex than that of the weak-inhibition regime. For this reason, we do not show systematically the codimension one bifurcation diagrams for each slice that can be identified in the whole codimension two diagrams, contrarily to what we did in the weak-inhibition regime. Nonetheless, we provide the codimension one diagrams in three different sample areas called A, B, C highlighted in Fig. (S7), and specifically for $I_I = -4$, $I_I = -13.25$ and $I_I = -16$.

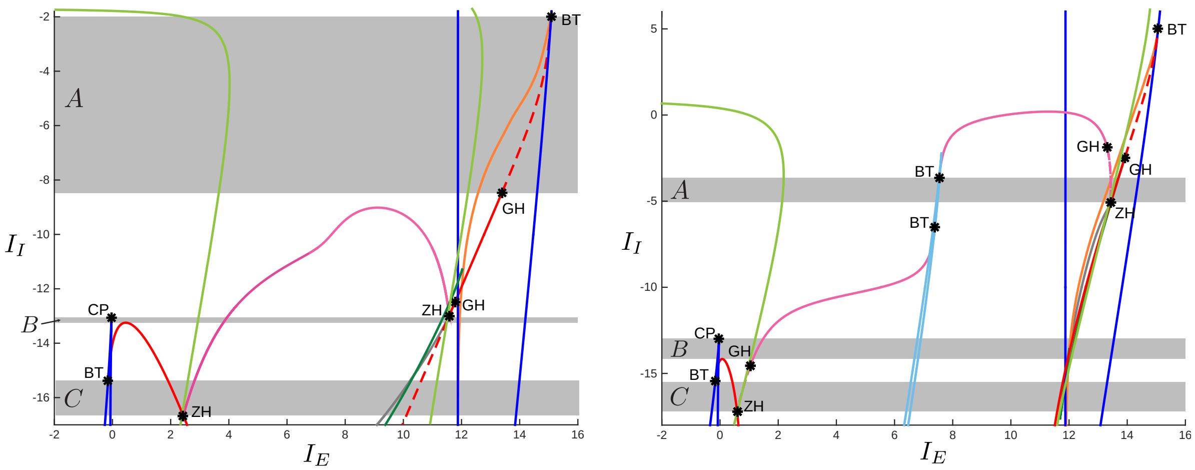


Figure S7: As in Fig. (S4), here we focus on the upper-half part of the codimension two bifurcation diagrams obtained for $J_{II} = -34$ (left), and $J_{II} = -100$ (right). Specifically, we identify three regions in both of them, represented by gray backgrounds, whose corresponding codimension one diagrams are shown in Figs. (S8) and (S9).

We underline that, nearby the graphs of $\mu_E = \mu_E(I_E)$, we show also that of $\mu_I = \mu_I(I_E)$. This choice is motivated by the fact that, unlike the weak-inhibition regime, now the secondary branches of equilibria exhibit qualitative differences in excitatory and inhibitory neurons. The collection of these diagrams is shown in Figs. (S8) and (S9).

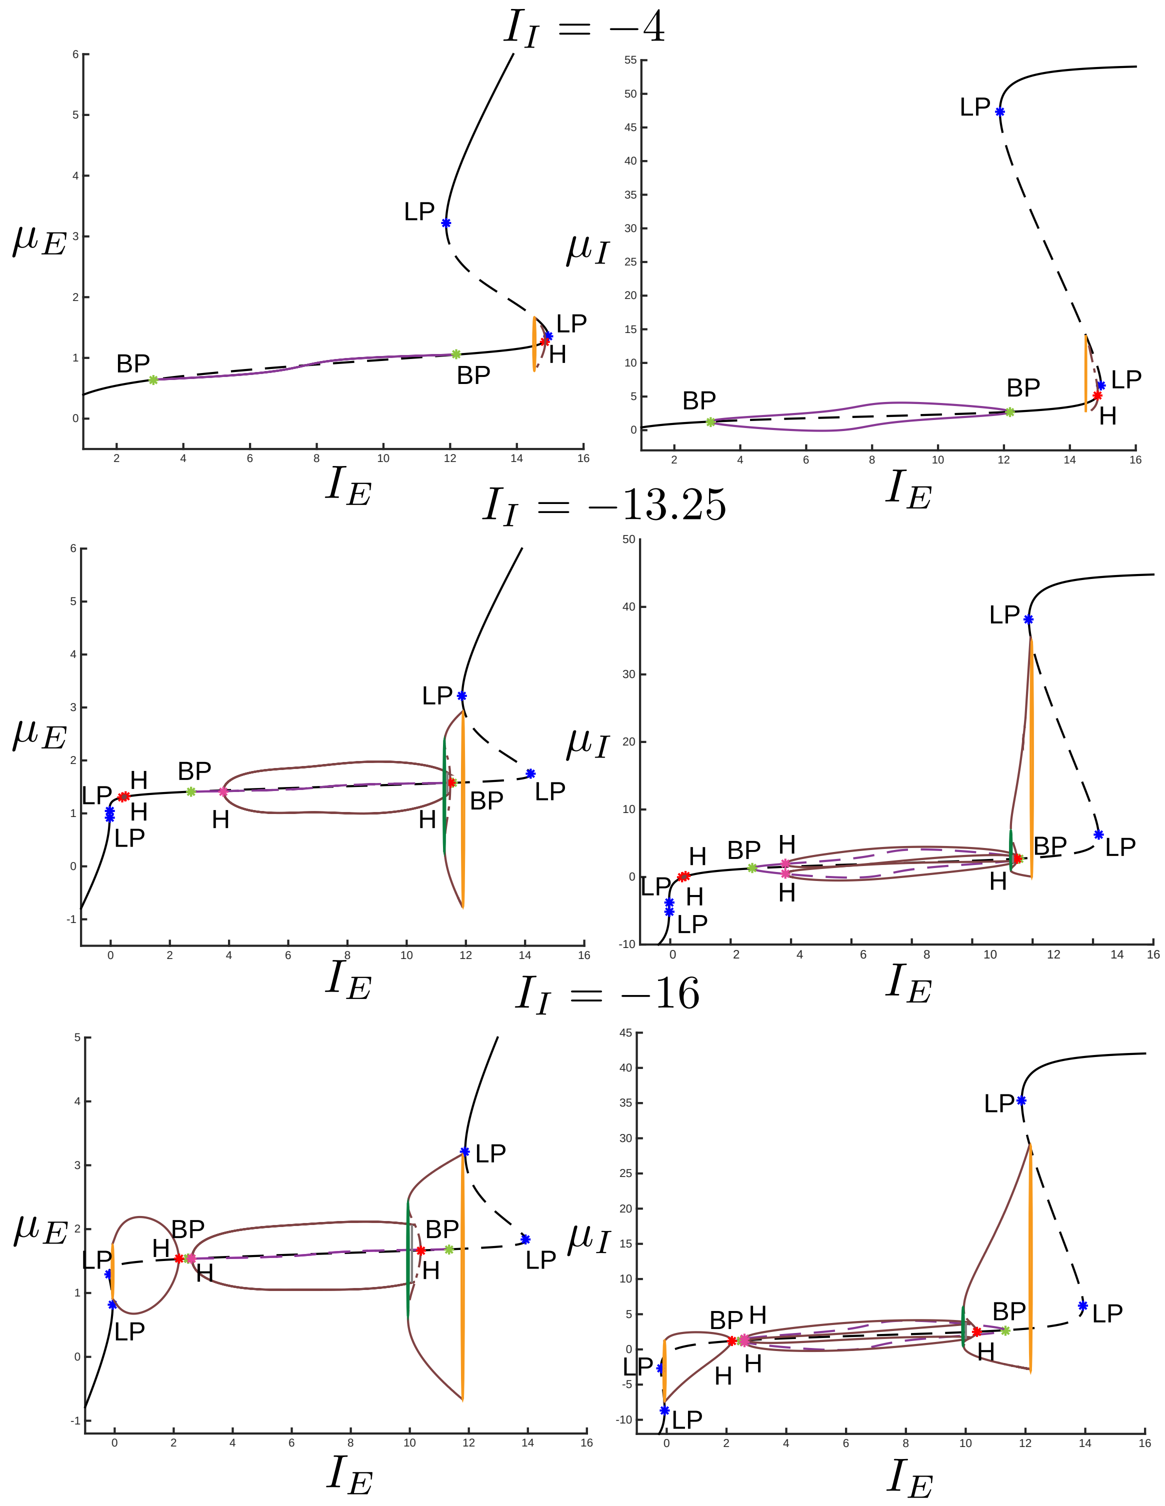


Figure S8: Each row of this figure describes $\mu_E$ and $\mu_I$ for $J_{II} = -34$ as a function of $I_E$, for three different values of $I_I$.

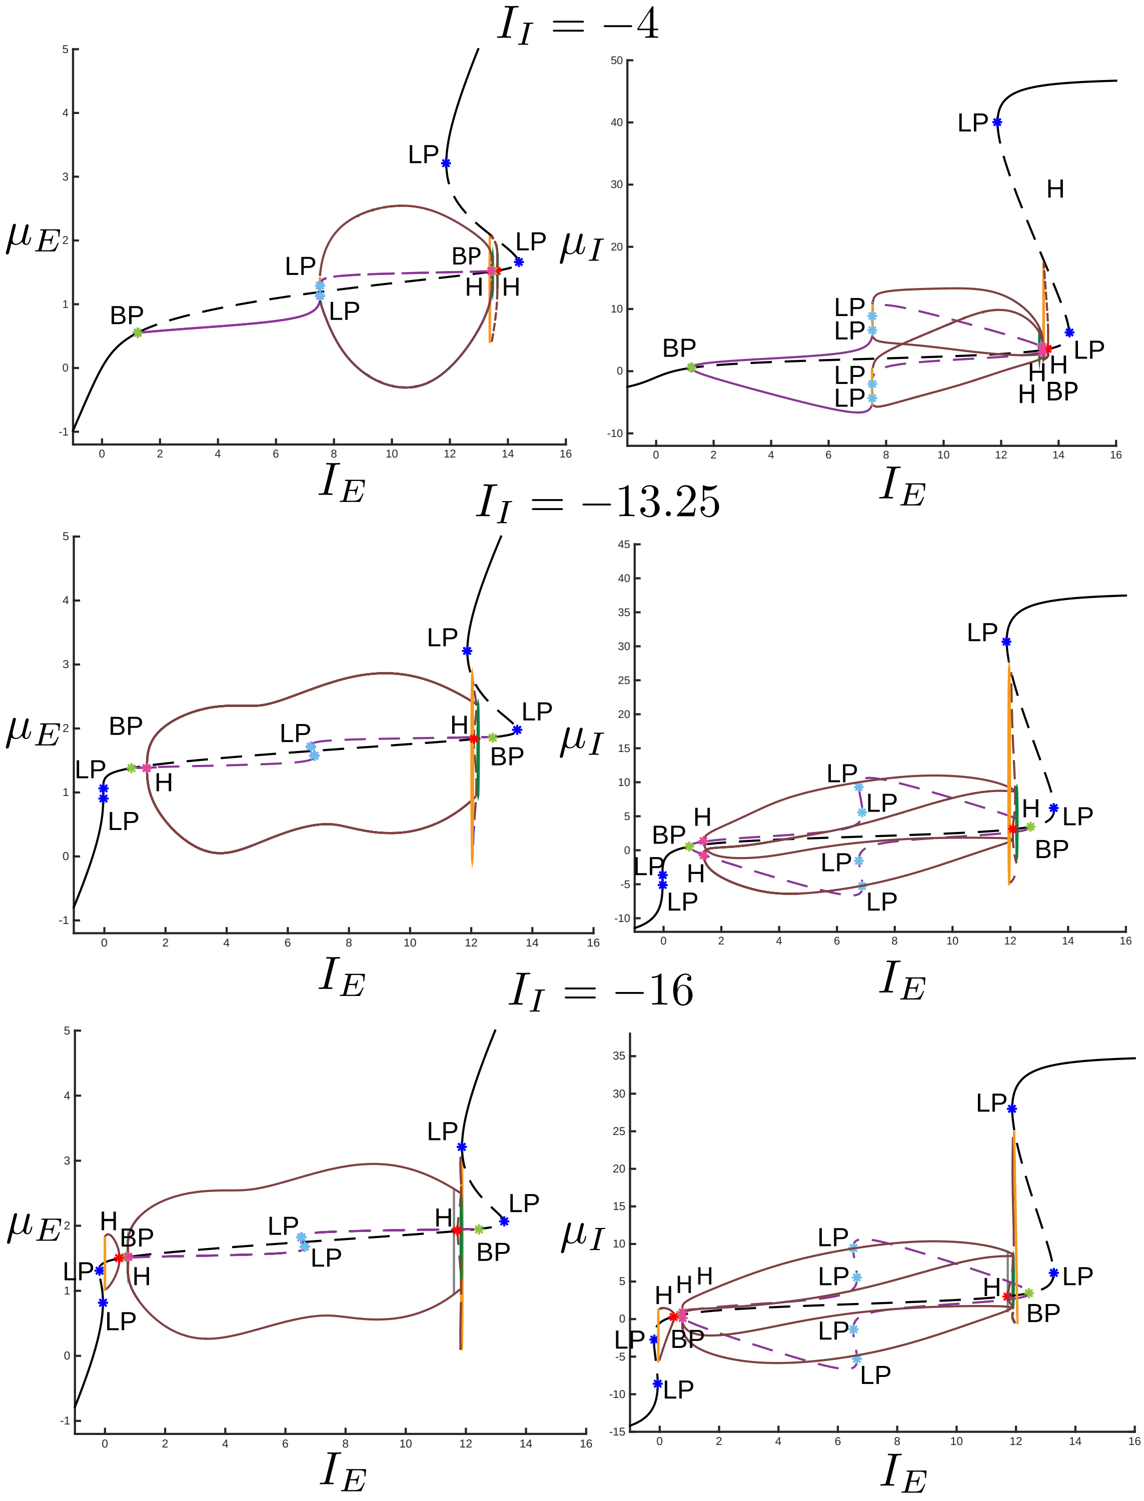


Figure S9: As in Fig. (S8), but for $J_{II} = -100$.

[**A**] The model exhibits non-oscillating or oscillating activity depending on the inhibitory strength. On the one hand, for $J_{II} = -34$ the model exhibits non-oscillating activity on both the primary and the secondary branches since stable limit cycles do not exist. The primary branch is characterized by stable foci (nodes) for low (high) values of $I_E$. These equilibria describe low and high-activity states, respectively. For intermediate values of $I_E$, the solutions of the model converge to the stable equilibria of the secondary branches. However, bistability is present. On the other hand, for $J_{II} = -100$ the Andronov-Hopf bifurcation gives rise to stable limit cycles that represent oscillating activity with frequencies from 0 Hz at the homoclinic bifurcation up to 89 Hz.

[**B**] For both $J_{II} = -34$ and $J_{II} = -100$, the system presents both stable equilibria (nodes and foci) and stable limit cycles. As before, stable equilibria describe states with high firing-rates for large $I_E$, while states with low firing-rates emerge for low $I_E$. Moreover, for intermediate values of $I_E$, the unstable equilibria of both the primary and secondary branches are surrounded by stable limit cycles. In particular, for $J_{II} = -34$, the high-amplitude stable oscillations produced by the Andronov-Hopf bifurcation on the primary branch exhibit frequencies from 0 Hz at the homoclinic bifurcation up to nearly 90 Hz. On the contrary, the low-amplitude oscillations originated from the secondary branches display frequencies from 124 to 154 Hz. For $J_{II} = -100$, the oscillations originated from the Andronov-Hopf bifurcation on the secondary branches span from 70 to 102 Hz.

[**C**] This third case turns out to be similar to the previous one. However, for both the inhibition strengths considered here, new stable limit cycles arise on the primary branch for low $I_E$, and vanish at the homoclinic bifurcation. In particular, for $J_{II} = -34$, their frequencies lie from 0 to 142 Hz. A similar frequency range (0-130 Hz) characterizes the limit cycles for high $I_E$. On the contrary, we find a narrow frequency range for the low-amplitude oscillations on the second branches (152-164 Hz). Finally, for $J_{II} = -100$, the oscillations on the primary branch exhibit frequency from 0 Hz at the homoclinic bifurcation to 73 Hz, while those on the secondary branches show frequency in the narrow range from 73 to 89 Hz. It is important to underline that, for both the inhibitory strengths, the high-frequency limit cycles display a torus bifurcation (gray line in Figs. (S8) and (S9)). Close to this bifurcation the spectrum of the oscillations contains two frequencies, therefore the neural network undergoes a quasiperiodic motion, as show in Fig. (S10).

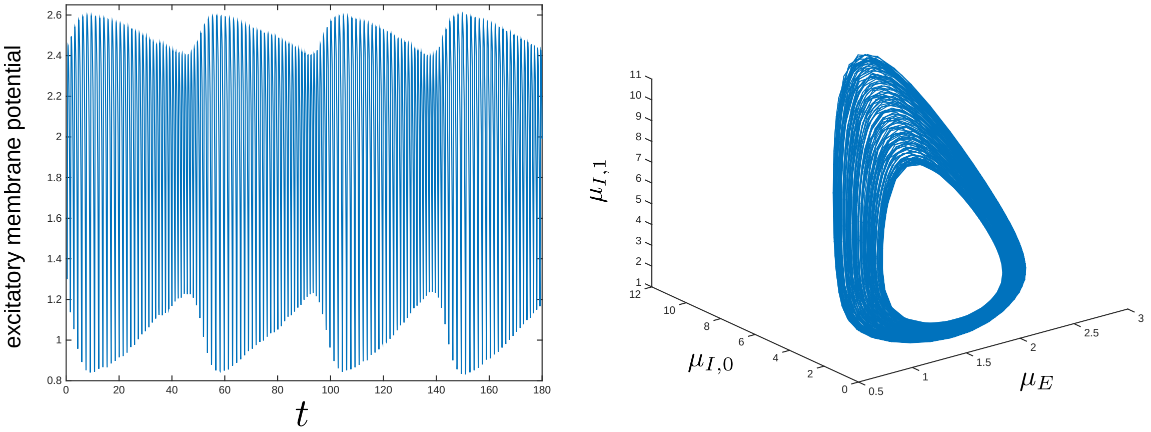


Figure S10: Time evolution of the excitatory membrane potentials at the torus bifurcation (left) and the corresponding trajectory in the phase space (right). Both the panels have been obtained for $J_{II} = -100$, $I_I = -16$ (area C in Fig. (S7)) and $I_E \approx 11.804$. From the left panel it is easy to see that the time evolution on the torus is characterized by two frequencies.

# References


[1] D. Fasoli, A. Cattani, and S. Panzeri. The complexity of dynamics in small neural circuits. arXiv:1506.08995 [q-bio.NC], 2015.

[2] C. Hermite. Sur la résolution de l'équation du cinquieme degré. *C. R. Acad. Sci.*, **46**: 508–515, 1858.

[3] J. Touboul, F. Wendling, P. Chauvel, and O. Faugeras. Neural mass activity, bifurcations, and epilepsy. *Neural Comput.*, **23**(12):3232–3286, 2011.

[4] H. R. Wilson and J. D. Cowan. Excitatory and inhibitory interactions in localized populations of model neurons. *Biophys J.*, **12**(1):1–24, 1972.

[5] P. Andersen and J. Eccles. Inhibitory phasing of neuronal discharge. *Nature*, **17**(196):645–647, 1962.

[6] W. J. Freeman. Analog simulation of prepyriform cortex in the cat. *Math. Biosciences*, **2**:181–190, 1968.

[7] W. J. Freeman. Patterns of variation in waveform of averaged evoked potentials from prepyriform cortex in cats. *J. Neurophysiol.*, **31**:1–13, 1968.

[8] M. Steriade, D. A. McCormick, and T. J. Sejnowski. Thalamocortical oscillations in the sleeping and aroused brain. *Science*, **262**:679–685, 1993.

[9] G. Buzsáki and A. Draguhn. Neuronal oscillations in cortical networks. *Science*, **304**:1926–1929, 2004.

[10] M. Diesmann, M.-O. Gewaltig, and A. Aertsen. Stable propagation of synchronous spiking in cortical neural networks. *Nature*, **402**:529–533, 1999.
